# Supplementary material for: A Unified View on Graph Neural Networks as Graph Signal Denoising
Source: arXiv:2010.01777 source file (2021-10-18)
Supplement: Supplementary file 2 [file appendix_experiments.tex]

\section{Experiments}

\subsection{Datasets}\label{apx:datasets}
In this section, we provide information of the datasets we used in the experiments as follows:
\begin{compactitem}
    \item {\bf Citation Networks:} \cora, \citeseer and \pubmed are widely adopted benchmarks of GNN models. In these graphs, nodes represent documents and edges denote the citation links between them. Each node is associated bag-of-words features of its corresponding document and also a label indicating the research field of the document.
    \item {\bf Co-purchase Graph:} \amazoncomp and \amazonphoto are co-purchase graphs, where nodes represent items and edges indicate that two items are frequently bought
together. Each item is associated with bag-of-words features extract from its corresponding reviews. The labels of items are given by the category of them.
\item {\bf Co-authorship Graphs:} \coauthorcs and \coauthorphys are co-authorship graphs, where nodes are authors and edges indicating the co-authorship between authors. Each author is associated with some features representing the keywords of his/her papers. The label of an author indicates the his/her most active research field.
    \item {\bf Blogcatalog:} \blogc is an online blogging community where bloggers can follow each other. The \blogc graph consists of blogger as nodes while their social relations as edges. Each blogger is associated with some features generated from key words of his/her blogs. The bloggers are labeled according to their interests.
    \item {\bf Flickr:} \flickr is an image sharing platform. The \flickr graph consists users as its nodes and the following relation among users as its edges. The users are labeled with the groups they joined. 
\item {\bf \airusa:} \airusa is a air traffic graph, where each node is an airport in the US. Two nodes are considered as connected if there existing commercial flights between them. Nodes are labeled with the the passenger flow of each airport. 
\end{compactitem}

Some statistics of these graphs are shown in Table~\ref{tab:statistics}. 
\begin{table}[!ht]
\small
\centering
\begin{tabular}{ccccc}
\toprule
                 & \#Nodes & \#Edges & \#Labels & \#Features  \\ \midrule
\cora             & 2708    & 13264   & 7        & 1433          \\ 
\citeseer         & 3327    & 12431   & 6        & 3703         \\ 
\pubmed           & 19717   & 108365  & 3        & 500          \\ 
\amazoncomp & 13381   & 504937  & 10       & 767           \\ 
\amazonphoto    & 7487    & 245573  & 8        & 745           \\ 
\coauthorcs      & 18333   & 182121  & 15       & 6805          \\ 
\coauthorphys  & 34493   & 530417  & 5        & 8415        \\ 
\blogc      & 5196    & 348682  & 6        & 8189          \\ 
\flickr  & 7575   & 487051  & 9      & 12047        \\ 
\airusa & 1190&28388 &4&238\\
\bottomrule
\end{tabular}
\caption{Dataset summary statistics.}
\label{tab:statistics}
\end{table}
\begin{figure*}[ht!]%
%\vskip -0.2em
     \centering
     \subfloat[\cora]{{\includegraphics[width=0.19\linewidth]{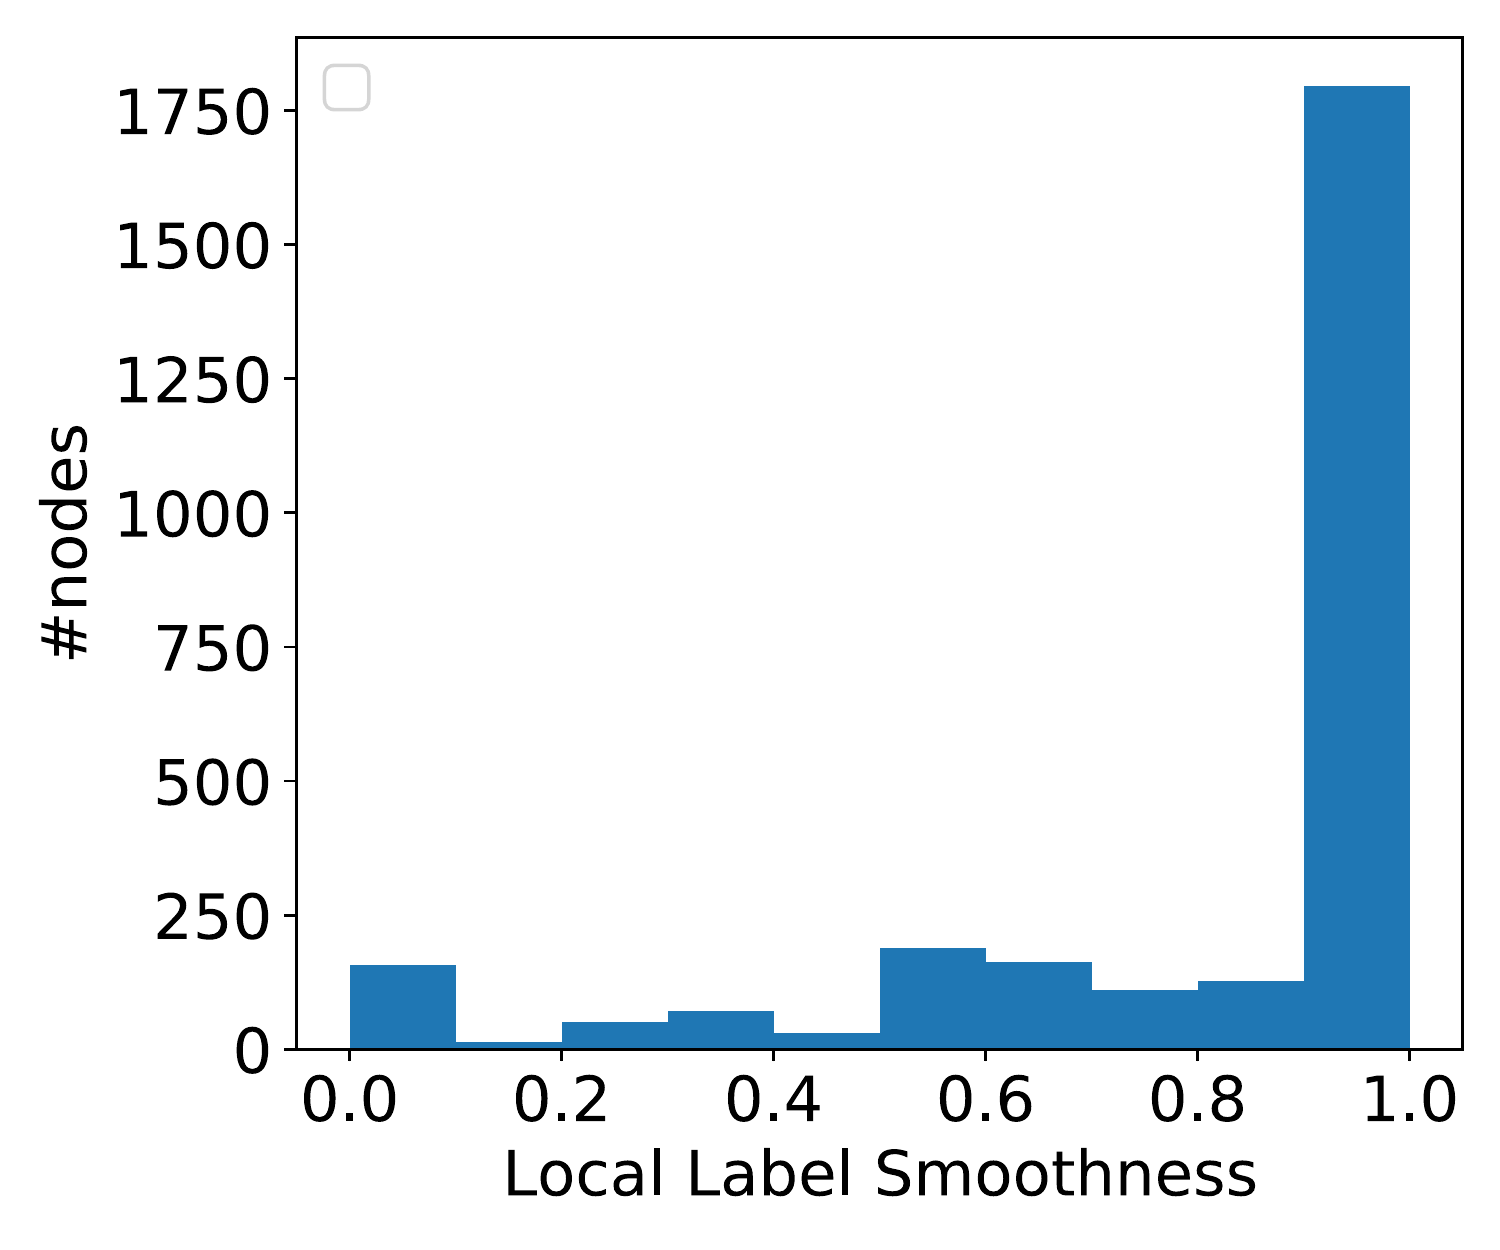} }}%
     \subfloat[\citeseer]{{\includegraphics[width=0.19\linewidth]{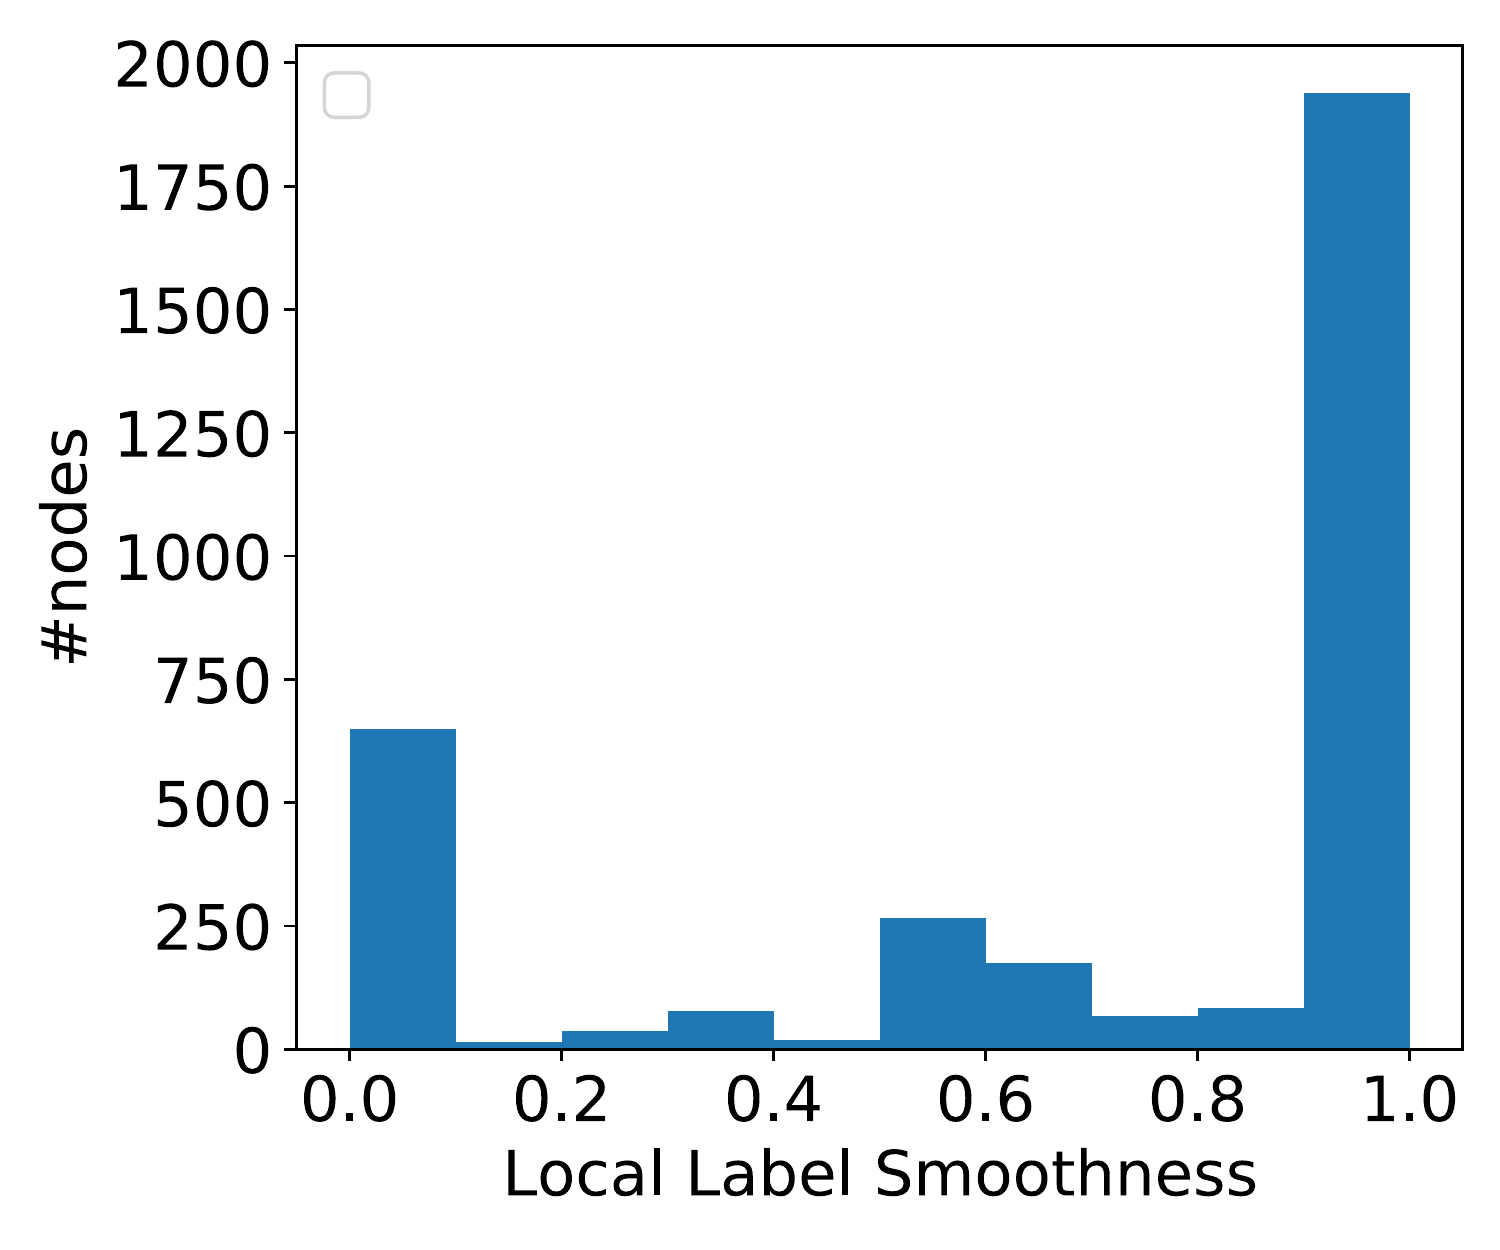} }}%
    \subfloat[\pubmed]{{\includegraphics[width=0.19\linewidth]{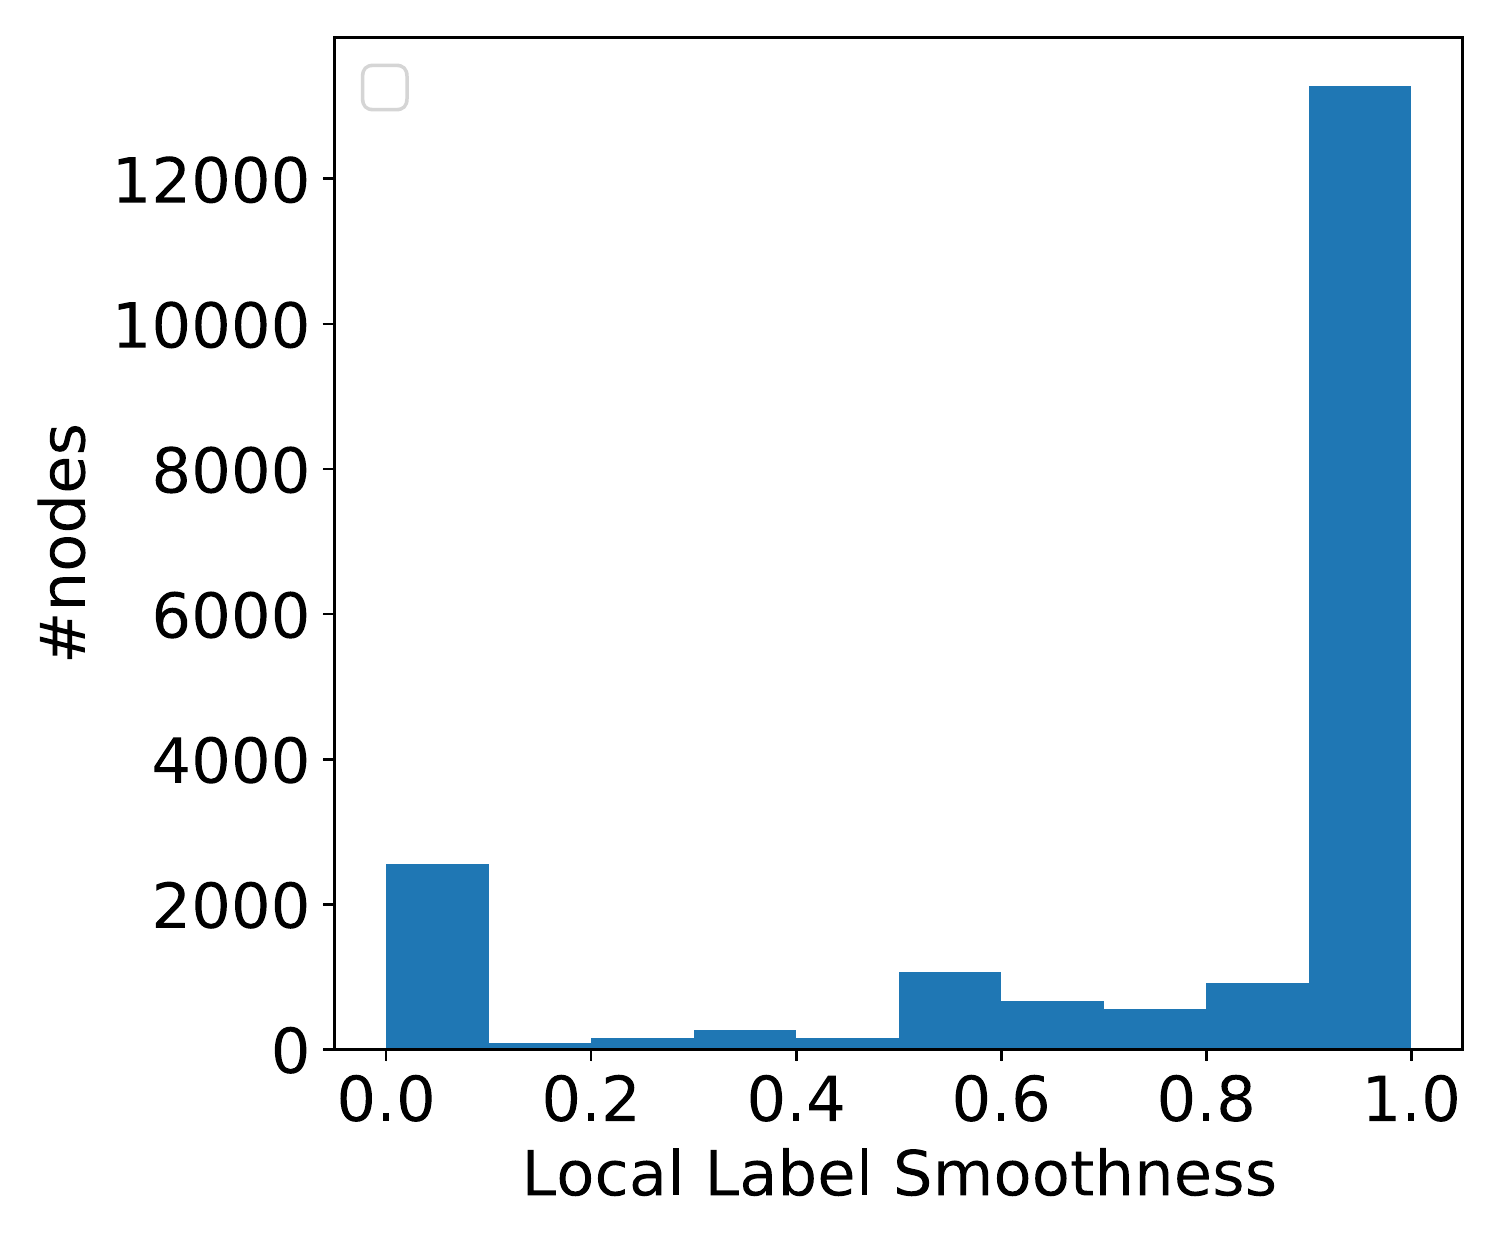} }}%
    \subfloat[\blogc]{{\includegraphics[width=0.19\linewidth]{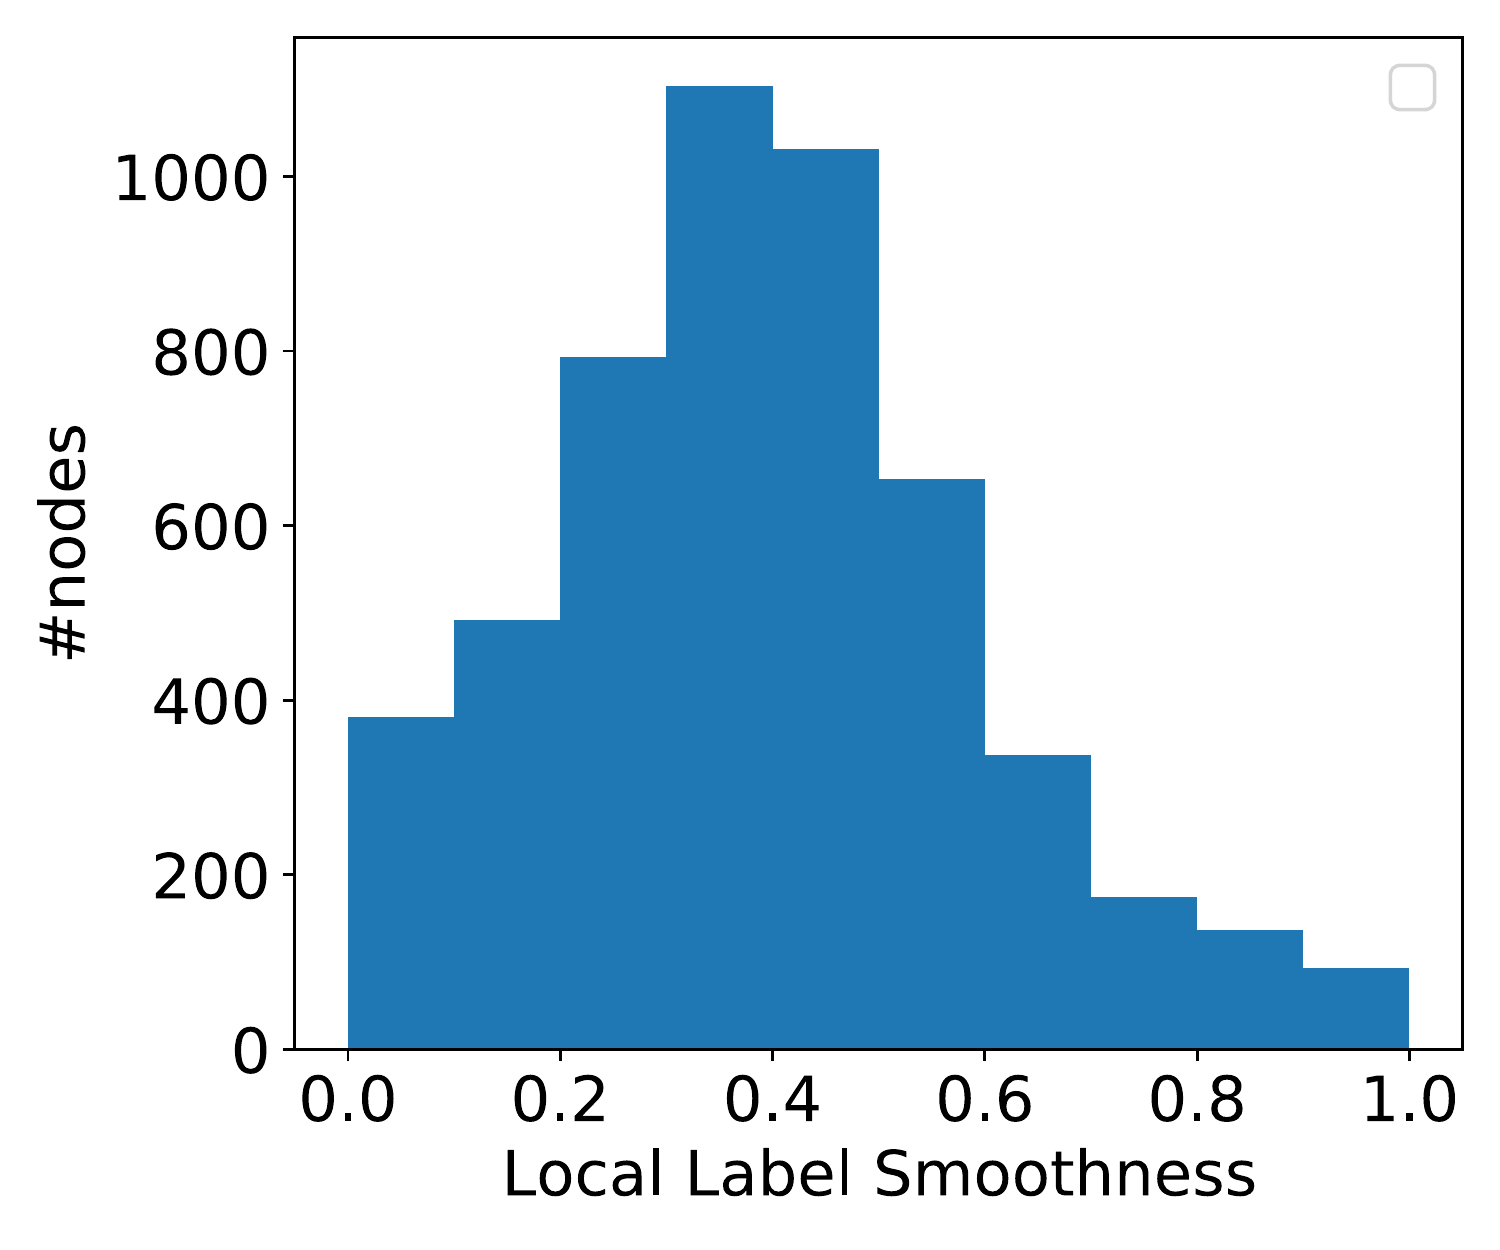} }}%
        \subfloat[\flickr]{{\includegraphics[width=0.19\linewidth]{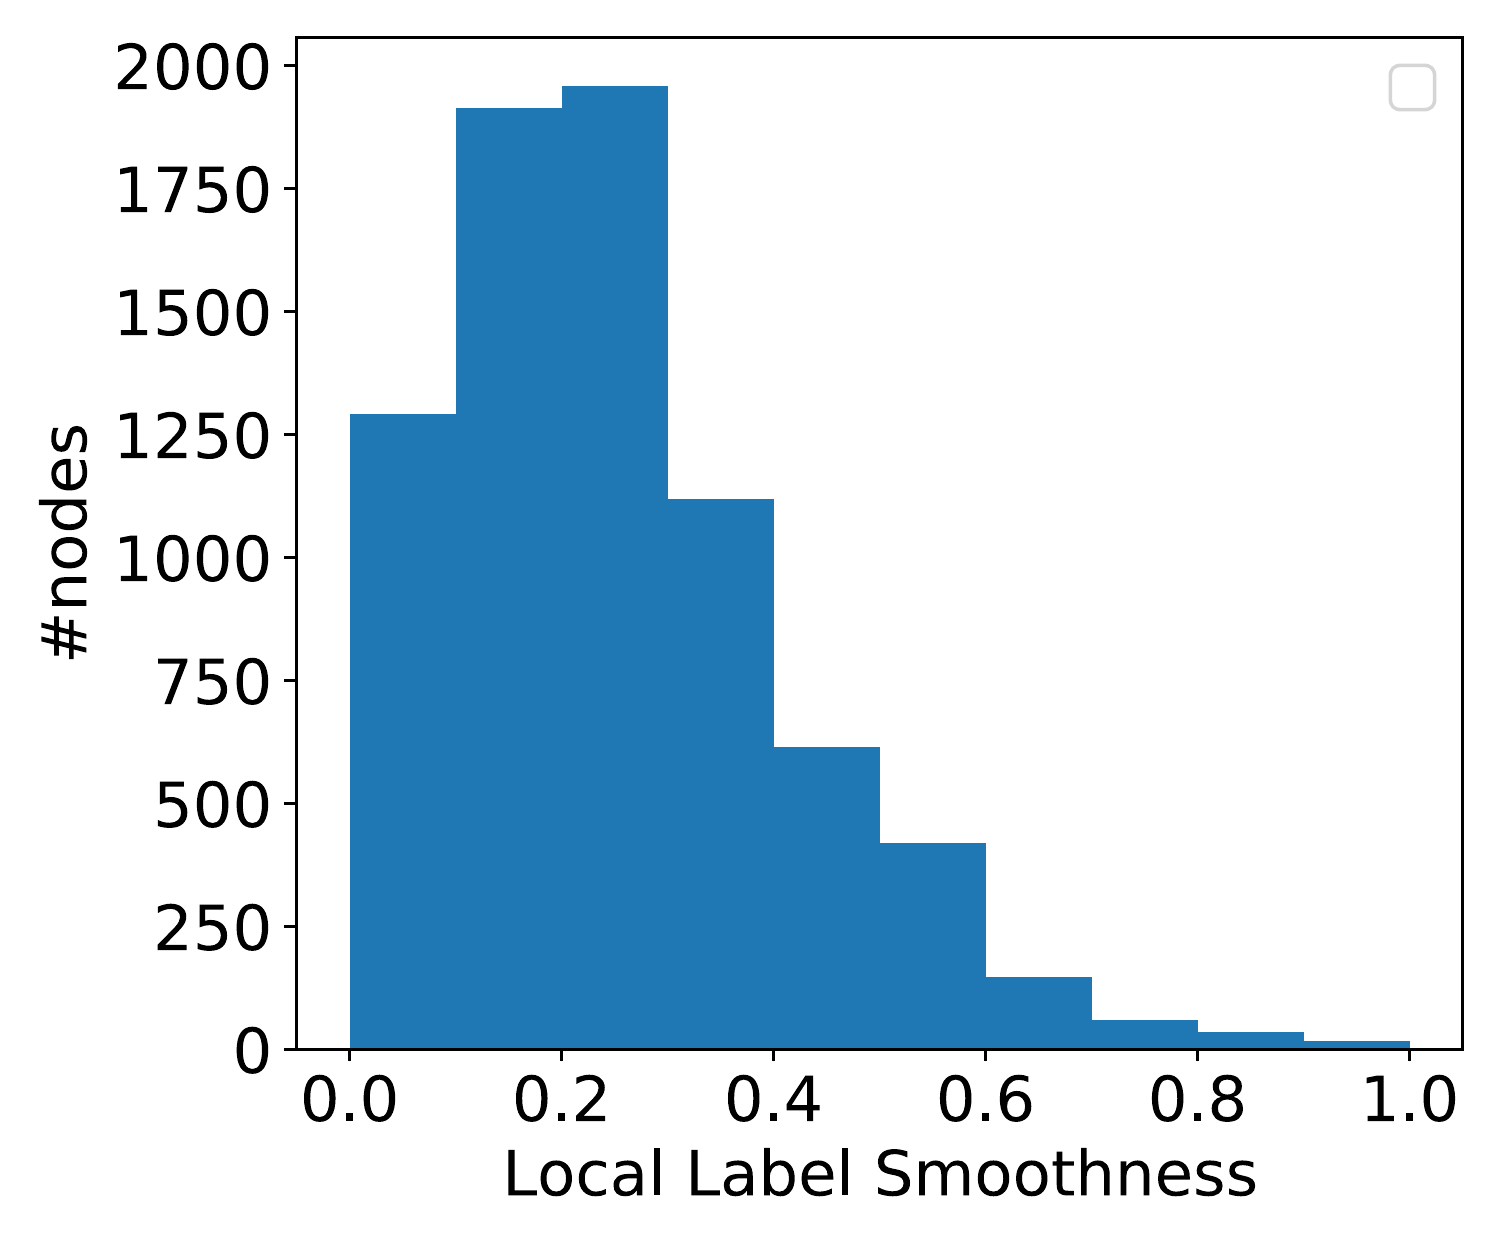} }\label{fig:flickr-alpha}}%

     \subfloat[\amazoncomp]{{\includegraphics[width=0.19\linewidth]{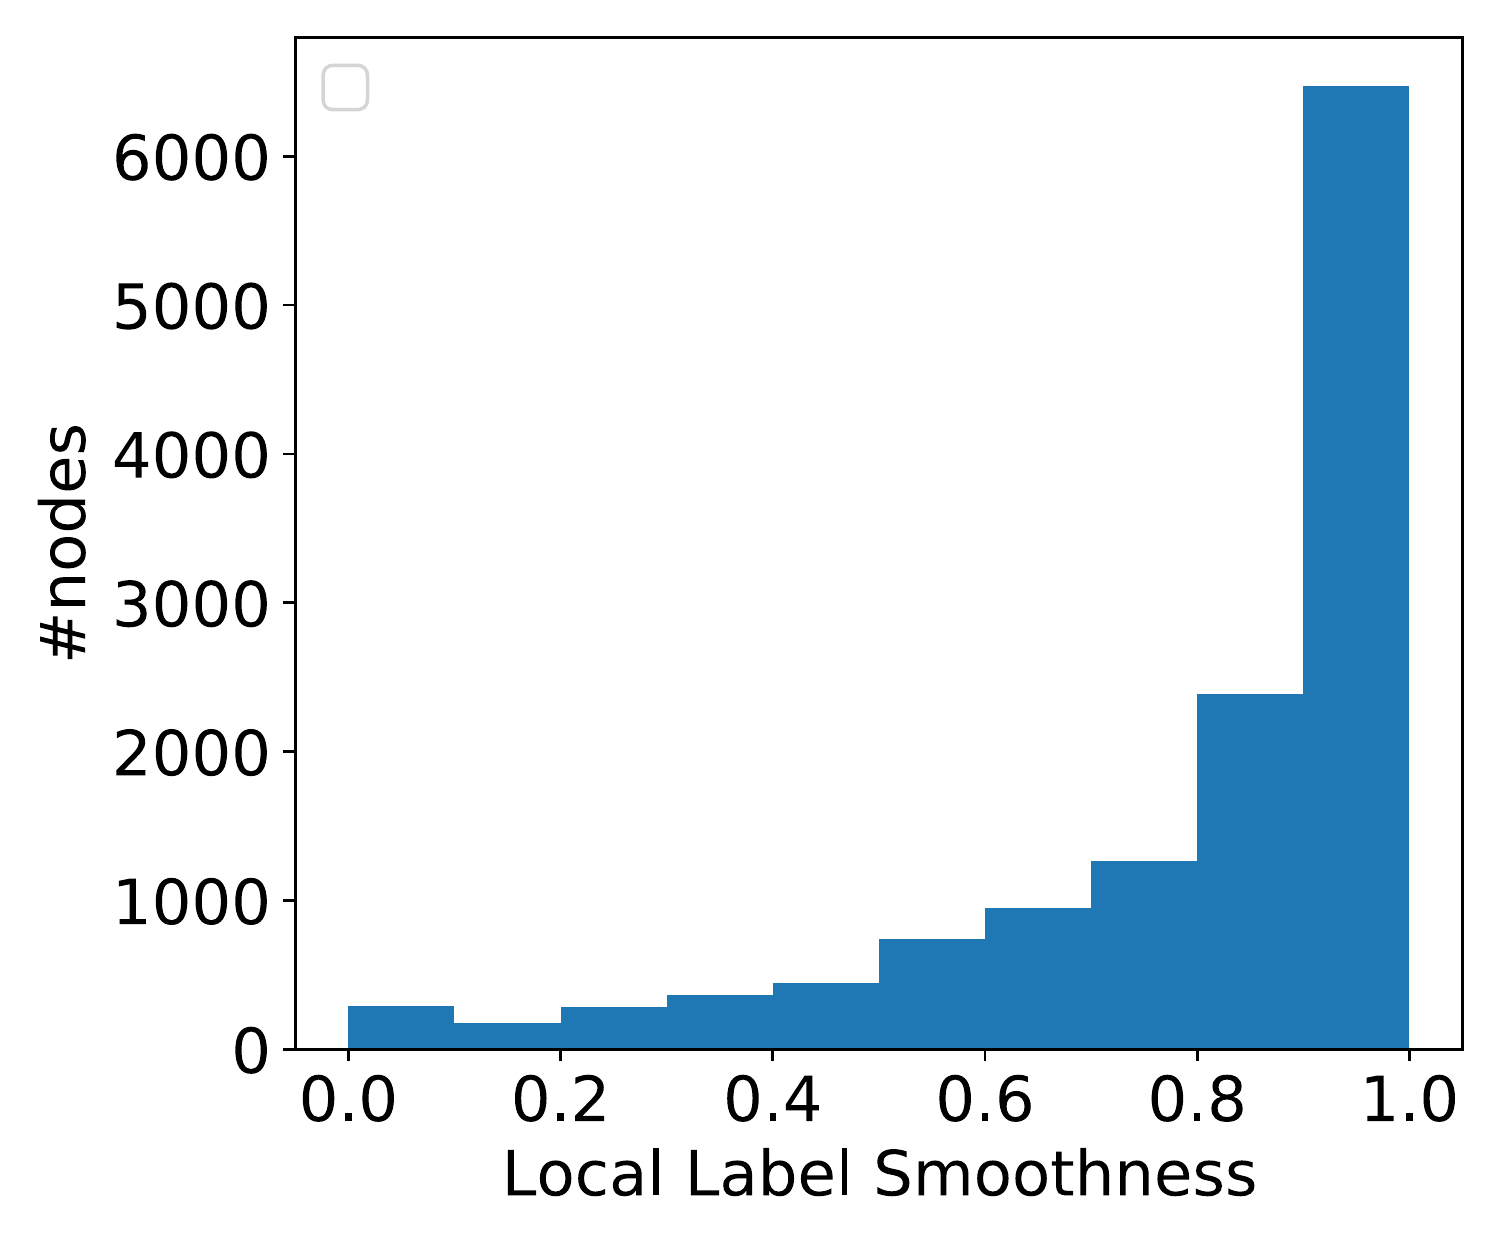} }}%
     \subfloat[\amazonphoto]{{\includegraphics[width=0.19\linewidth]{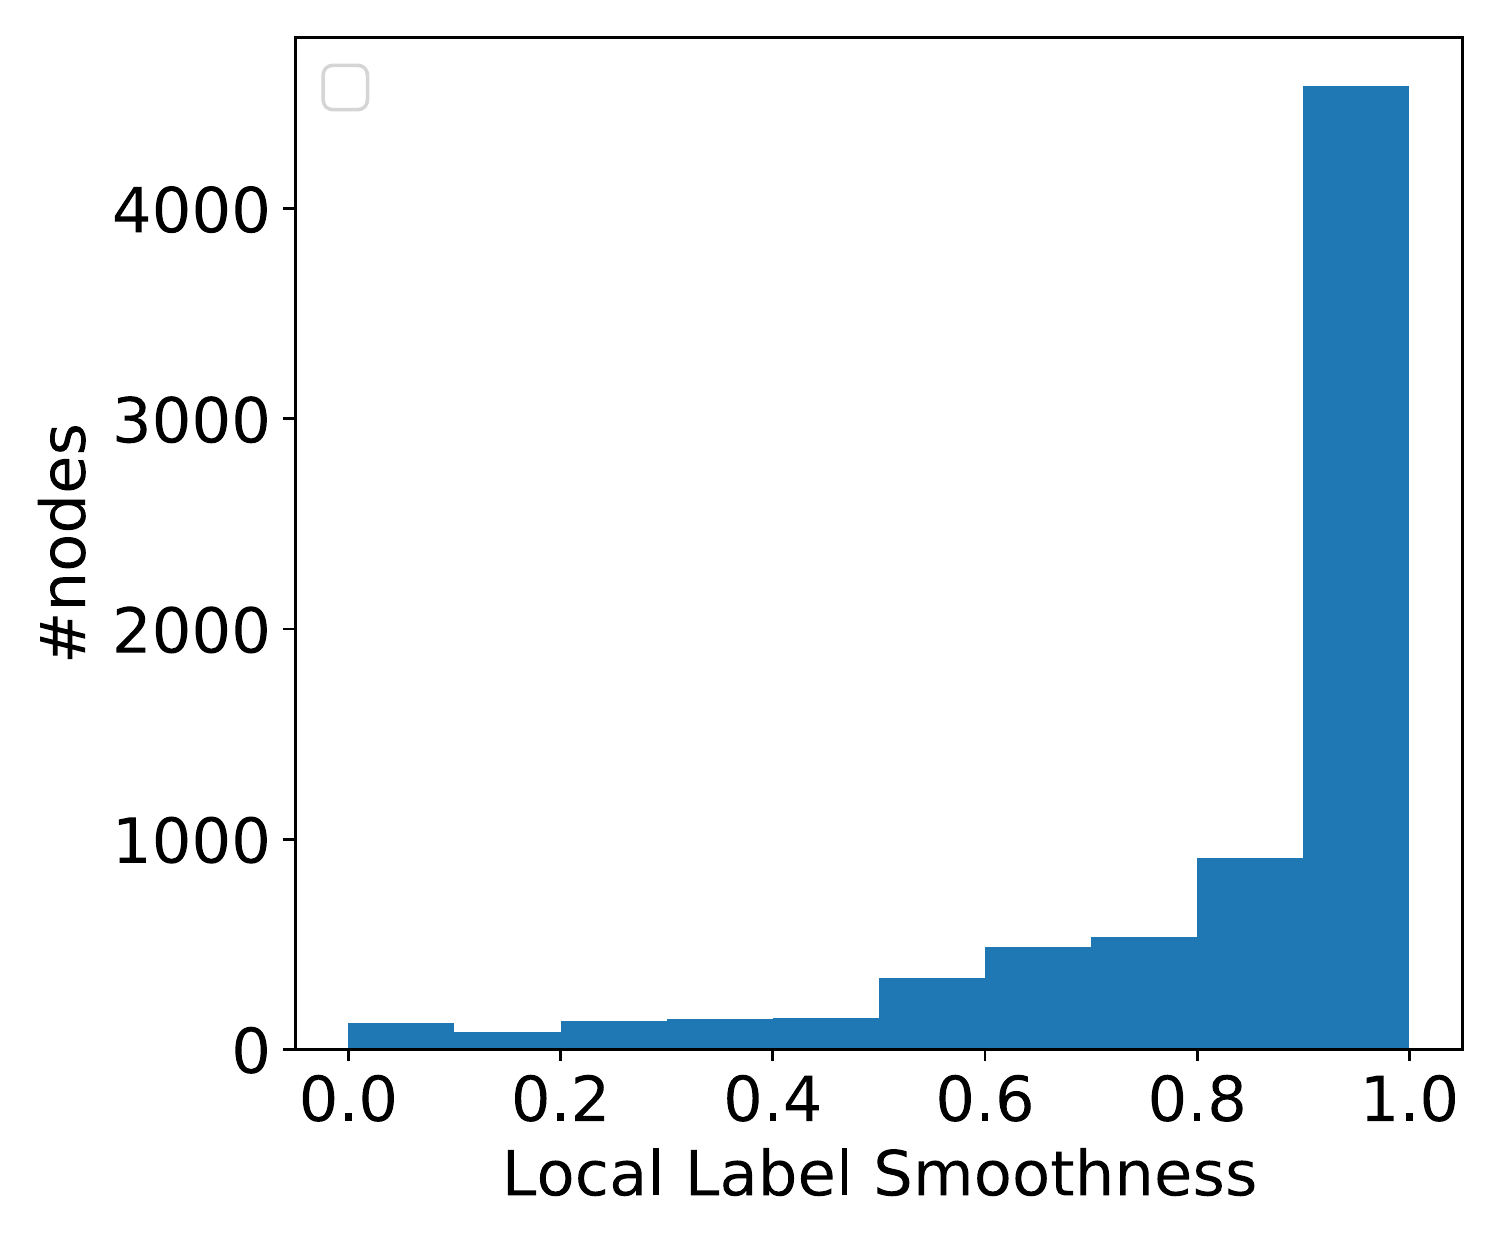} }}%
    \subfloat[\coauthorcs]{{\includegraphics[width=0.19\linewidth]{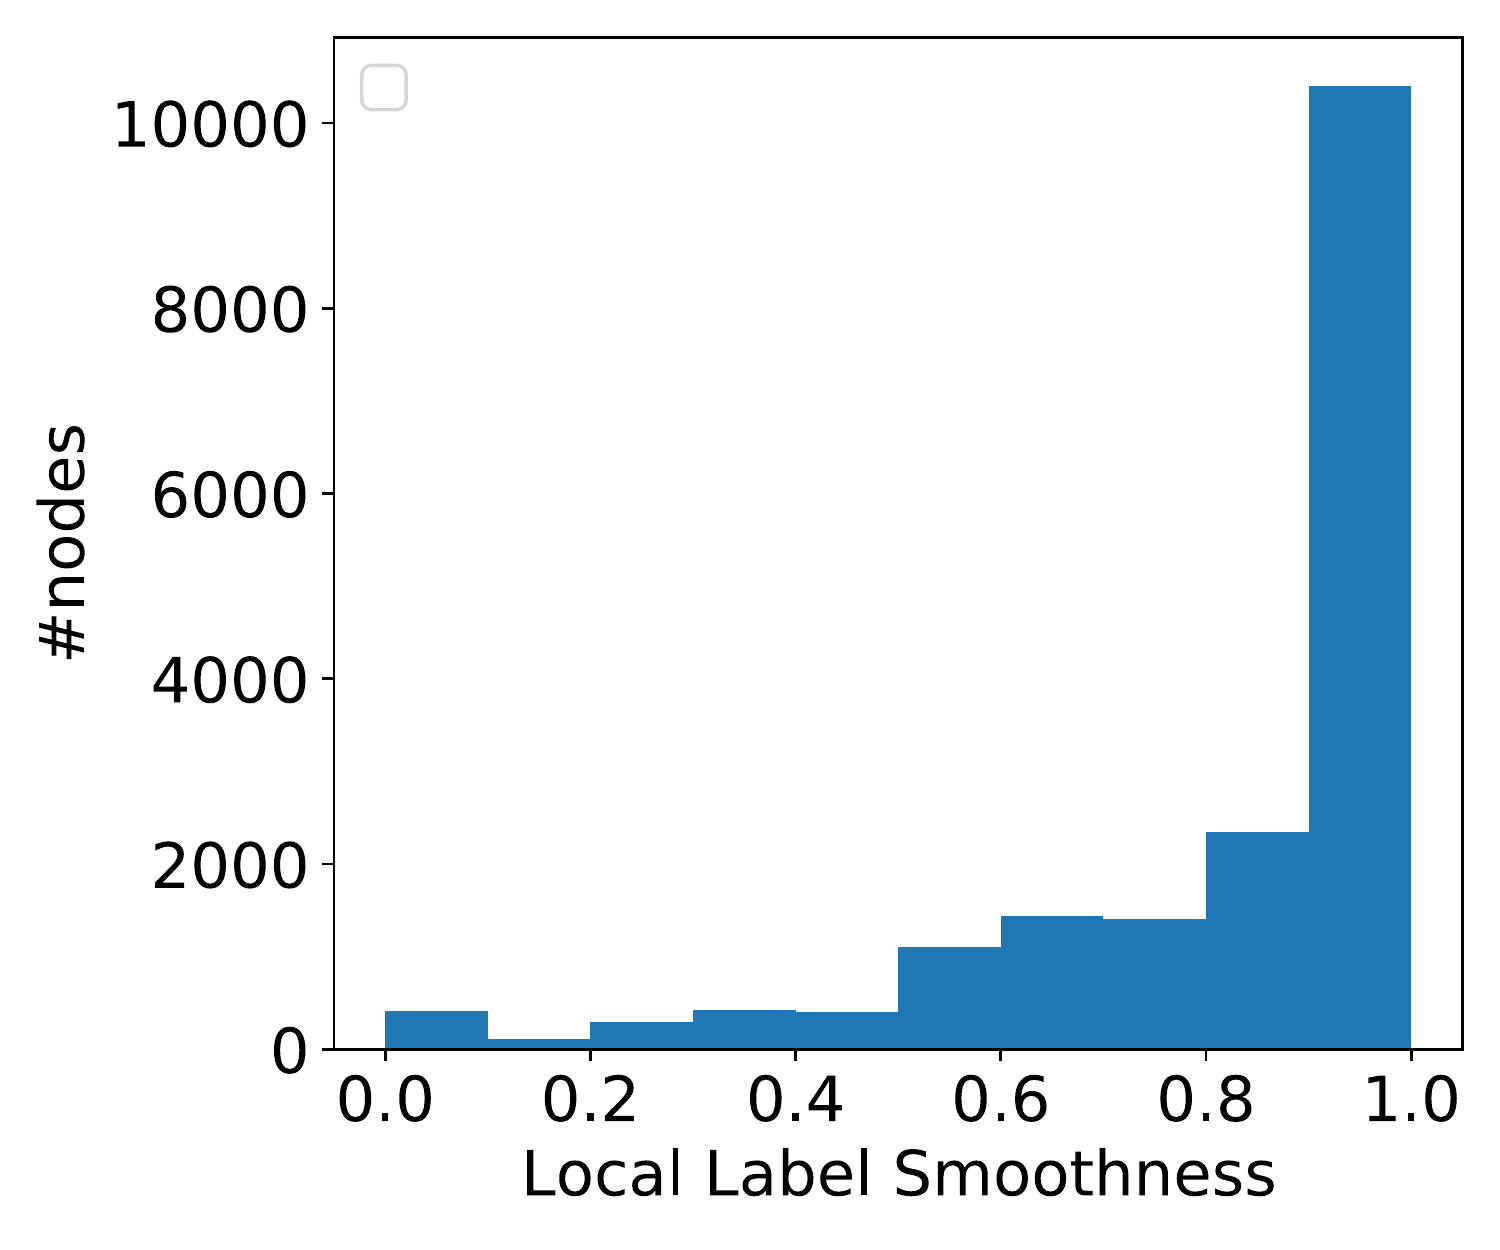} }}%
    \subfloat[\coauthorphys]{{\includegraphics[width=0.19\linewidth]{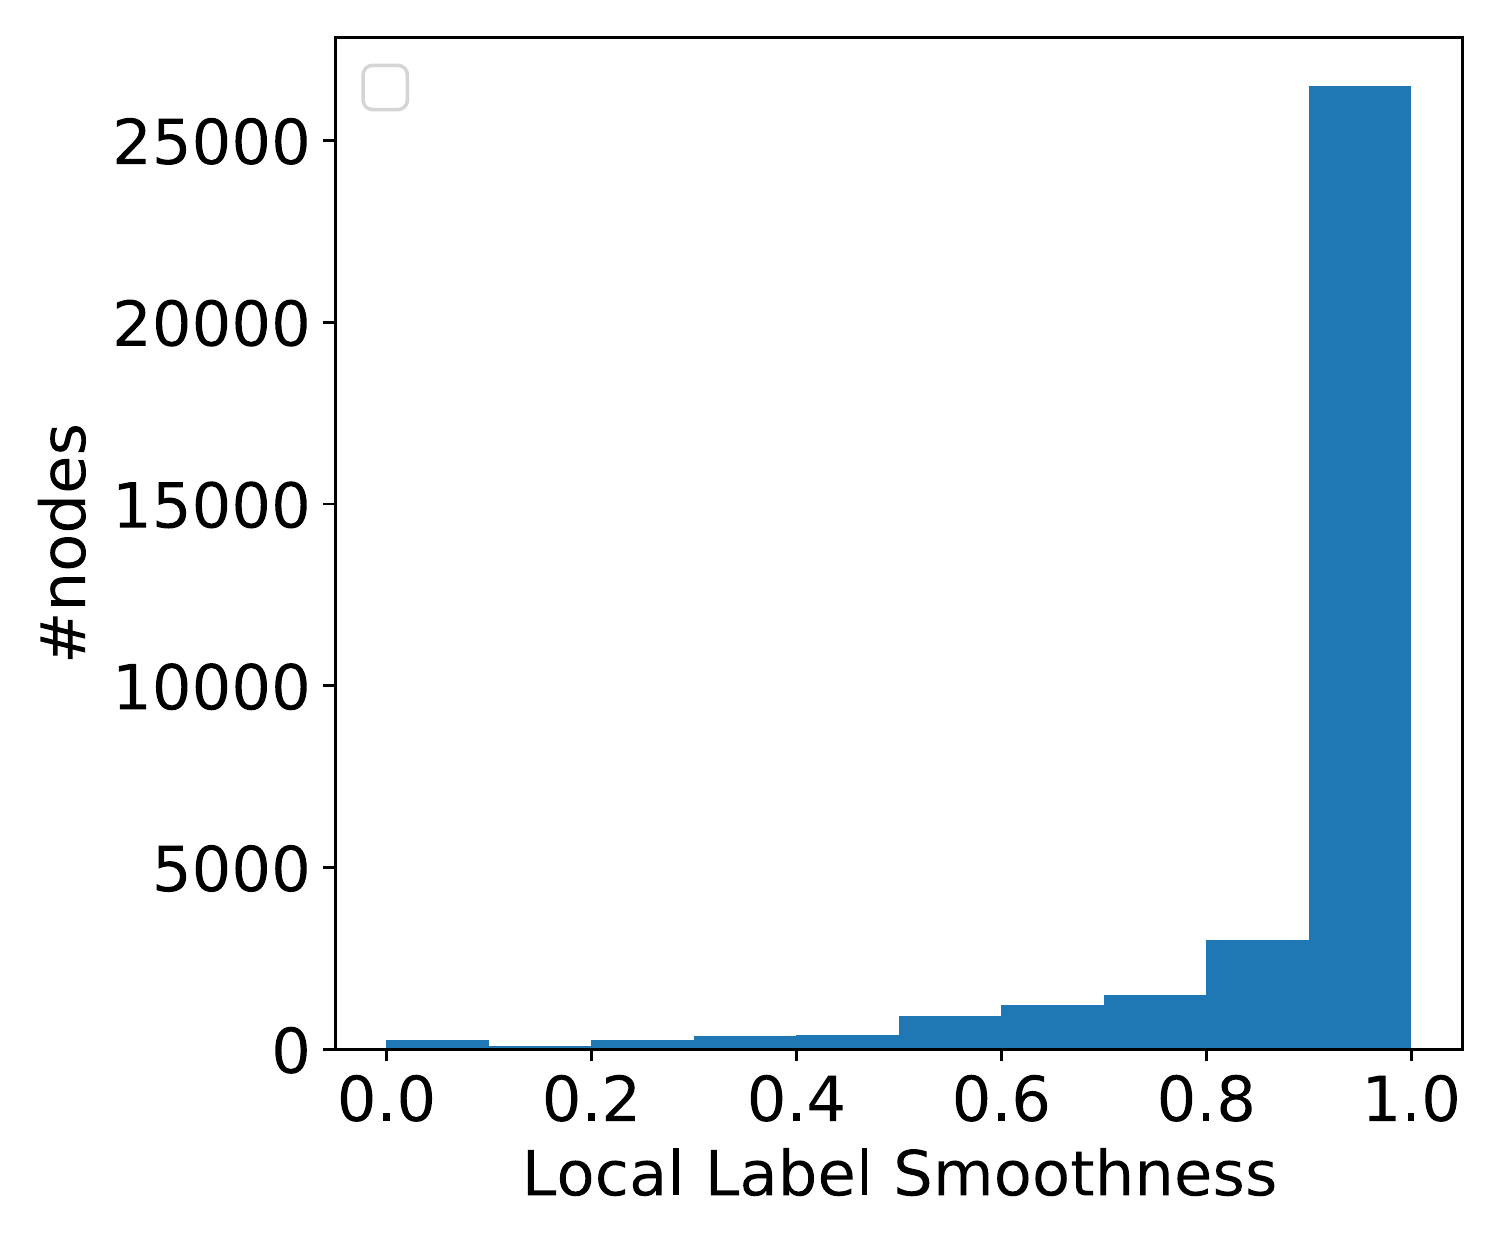} }}%
    \subfloat[\airusa]{{\includegraphics[width=0.19\linewidth]{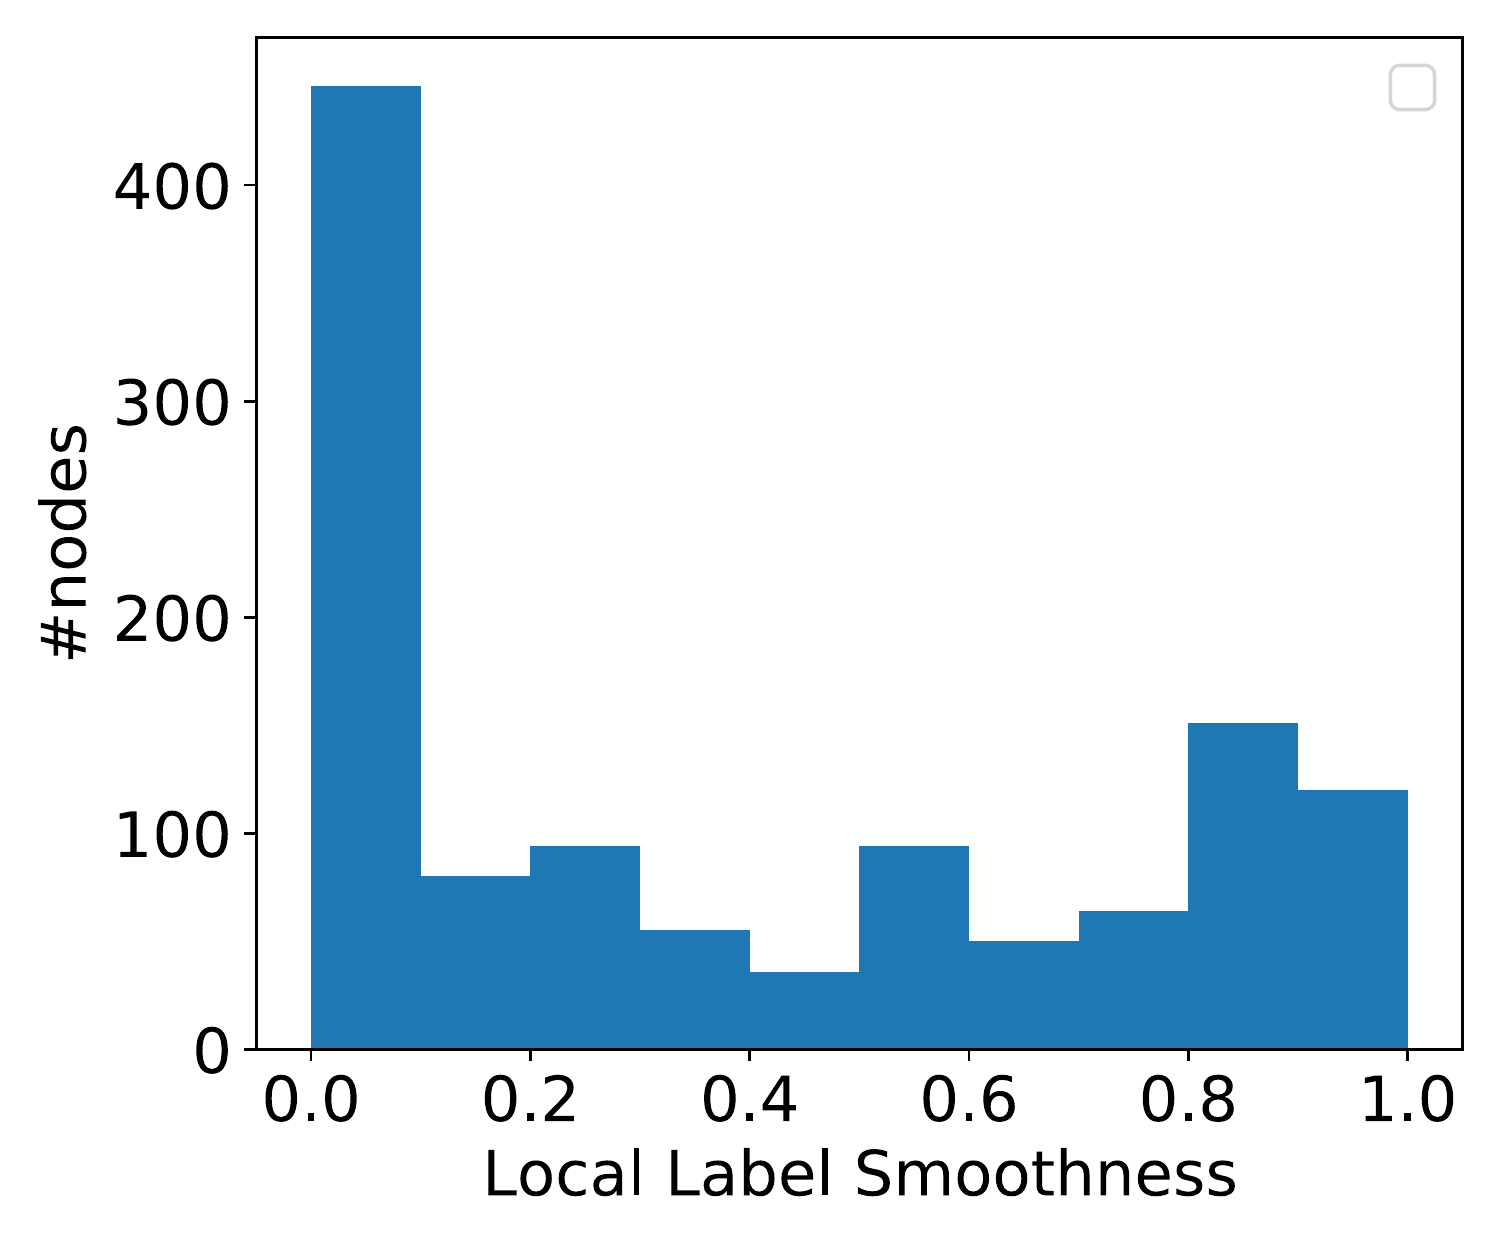} }}%
    \qquad
    \vskip -0.25em
    \caption{Distribution of local label smoothness (homophily) on different graph datasets: note the non-homogeneity of smoothness values.} 
    \label{fig:localsmoothness}
\vskip -0.25em
\end{figure*}
\subsubsection{Local Label Smoothness of Datasets} \label{apx:local_smooth}
We further present the distribution of local label smoothness in these datasets. For a node $v_i$ we formally define the local label smoothness as follows  
\begin{align}
    \text{ls}(i) = \frac{\sum\limits_{j\in \mathcal{N}(i)} \mathbf{1}\{ l(i) =l(j)\}}{|{\mathcal{N}}(i)|}\label{eq:local_label_smooth}
\end{align}
where $l(v_i)$ denotes the label of node $v_i$ and $\mathbf{1}\{a\}$ is an indicator function, which takes $1$ as output only when $a$ is true, otherwise $0$. The distributions of local label smoothness for all $8$ datasets are presented in Figure~\ref{fig:localsmoothness}.

\subsection{Parameter Tuning}\label{apx:parameter}
 For all methods, we tune the hyperparameters from the following options: 1) learning rate: $\{0.005, 0.01,0.05\}$; 2) weight decay  $\{5{e-}04,5{e-}05,5{e-}06,5{e-}07,5{e-}08\}$; and 3) dropout rate: $\{0.2,0.5,0.8\}$. For APPNP and our method \methodadaptive, we further tune the number of iterations $K$ and the upper bound $s$ for $c_i$ in Eq.~\eqref{eq:cal_ci} from the following range: 1) $K$: $\{2, 5,10\}$; and $s$: $\{1,9,19,29\}$. Note that we treat APPNP as a special case of our proposed method with $\mathcal{C}_i=s$ in Eq.~\eqref{eq:cal_ci}.

% \subsection{Node Classification Accuracy For Nodes with Low-level and High-level Local Label Smoothness}\label{apx:low-high}
% The performance of nodes with low local label smoothness and high local label smoothness in \citeseer, \pubmed, \amazonphoto and \coauthorphys are presented in Figure~\ref{fig:remaining}.

% \begin{figure}[t!]%
% %\vskip -0.2em
%      \centering
%      \subfloat[\citeseer]{{\includegraphics[width=0.22\linewidth]{figs/lh_citeseer.pdf} }\label{fig:param-alpha}}%
%     \subfloat[\pubmed]{{\includegraphics[width=0.22\linewidth]{figs/lh_pubmed.pdf} }\label{fig:param-alpha}}%
%      \subfloat[\amazonphoto]{{\includegraphics[width=0.22\linewidth]{figs/lh_amazon-ph.pdf} }\label{fig:param-alpha}}%
%     \subfloat[\coauthorphys]{{\includegraphics[width=0.22\linewidth]{figs/lh_co-ph.pdf} }\label{fig:param-alpha}}%
%     \qquad
%     \vskip -0.25em
%     \caption{Accuracy with low label smoothness and high label smoothness nodes.  Note the consistent improvement in low smoothness cases, enabled by adaptive local smoothing.} 
%     \label{fig:remaining}
% \vskip -0.25em
% \end{figure}

\subsection{Local Smoothness Distribution of Attacked Graph}\label{apx:local_smooth_attack}
Graph adversarial attacks tend to connect nodes from different classes while disconnect nodes from the same class, which typically leads to more diverse distributions of local smoothness level. We present the distributions of the graphs generated by Mettack \citep{zugner2019adversarial} with different perturbation rate for \cora, \citeseer and \pubmed in Figure~\ref{fig:cora-localsmoothness}, Figure~\ref{fig:citeseer-localsmoothness} and Figure~\ref{fig:pubmed-localsmoothness}, respectively.
\begin{figure*}[t!]%
%\vskip -0.2em
     \centering
     \subfloat[0\%]{{\includegraphics[width=0.22\linewidth]{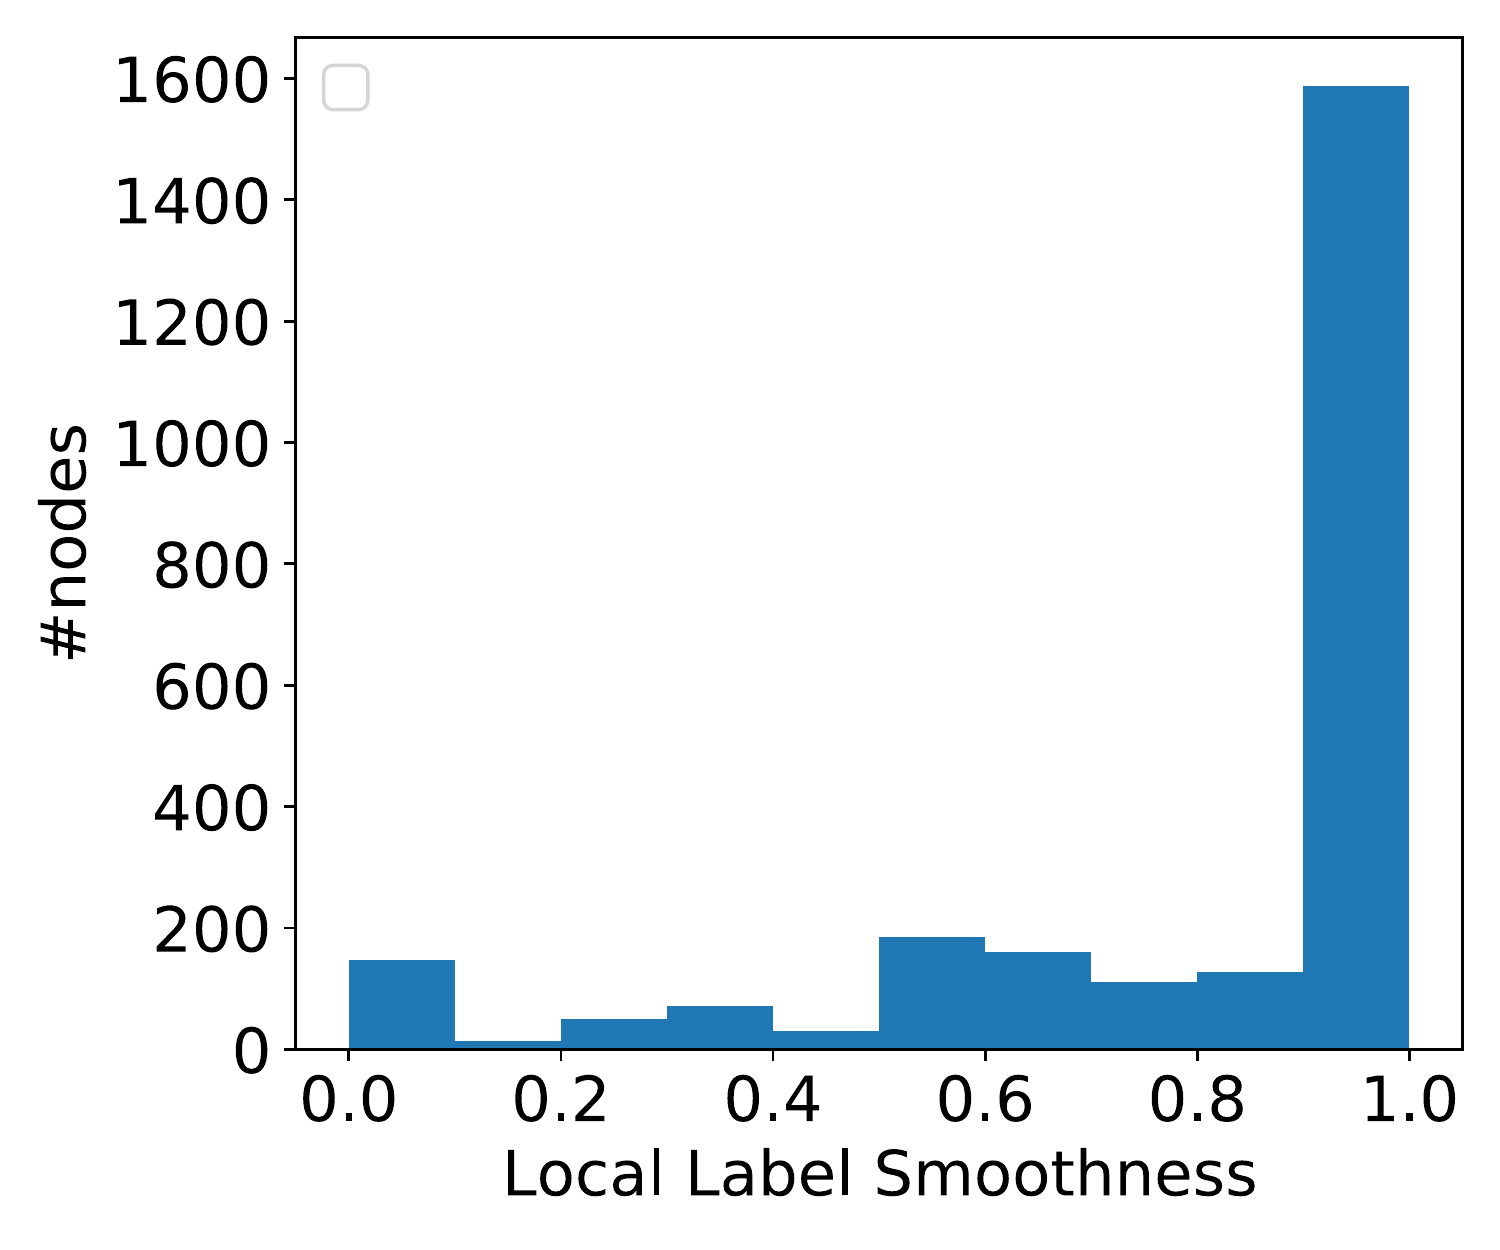}}}%
     \subfloat[5\%]{{\includegraphics[width=0.22\linewidth]{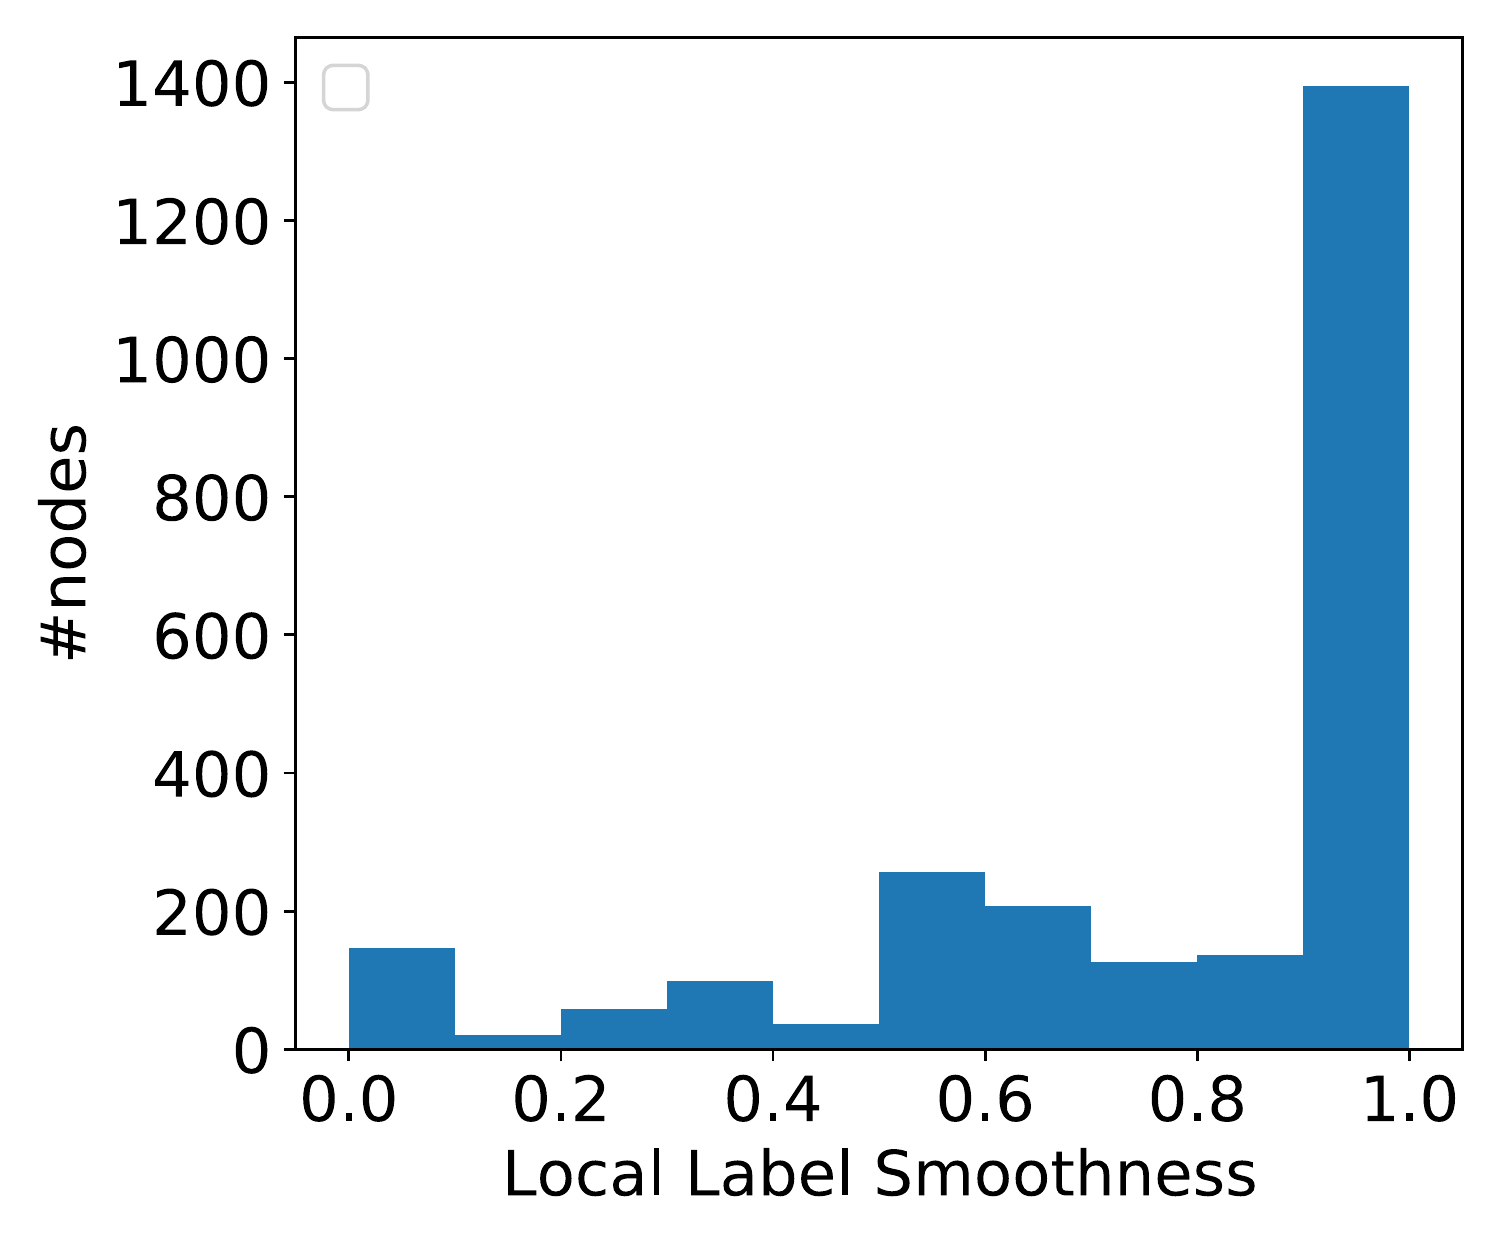} }}%
    \subfloat[15\%]{{\includegraphics[width=0.22\linewidth]{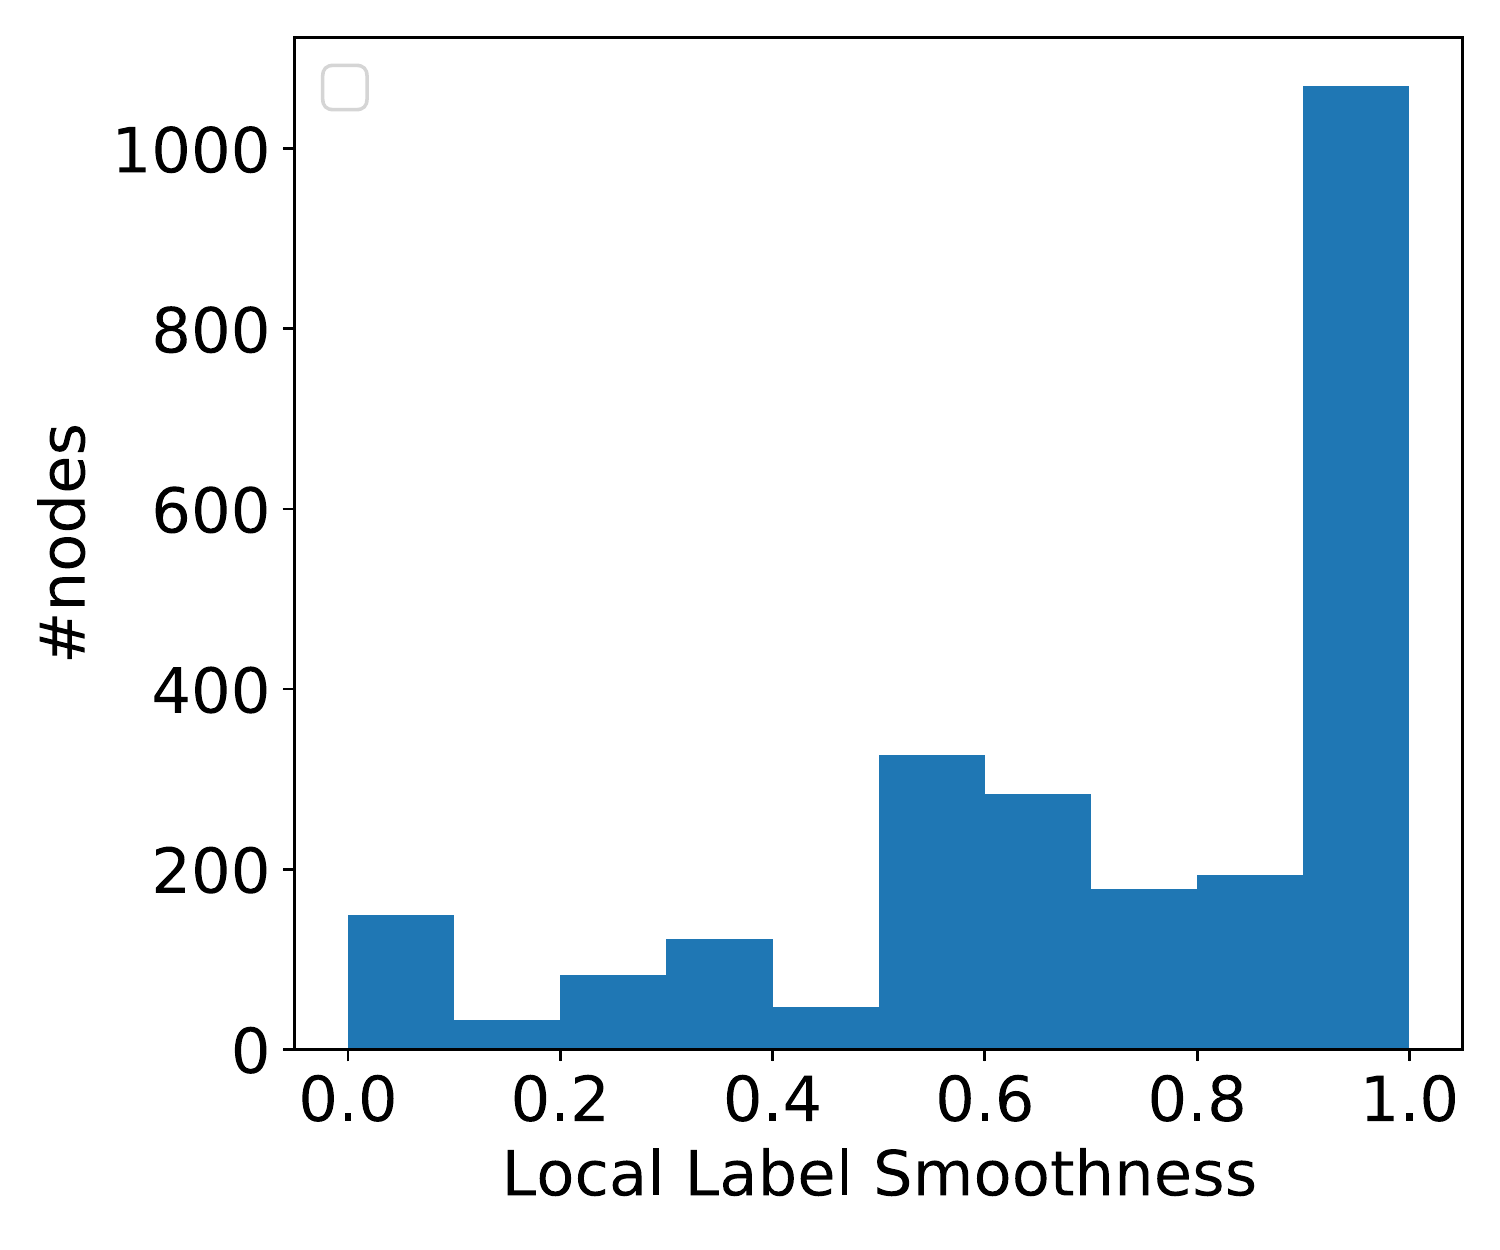} }}%
    \subfloat[25\%]{{\includegraphics[width=0.22\linewidth]{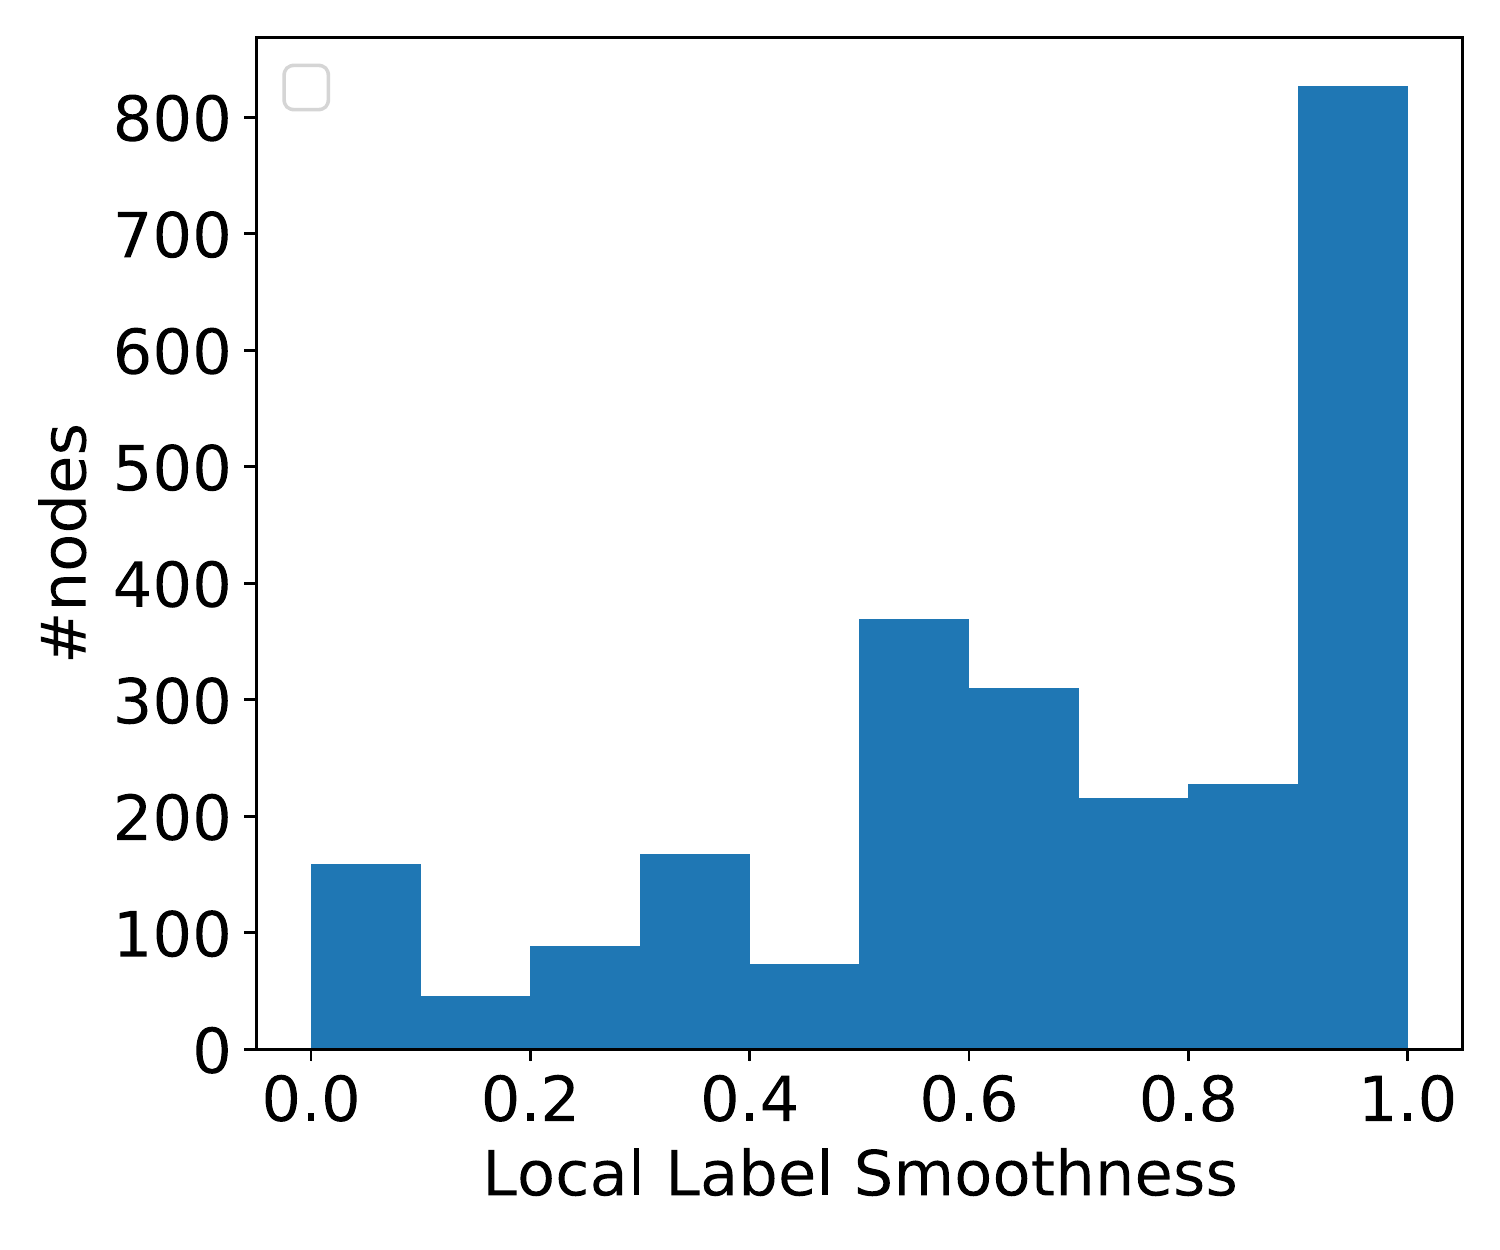} }}%
    \qquad
    \caption{Distribution of local label smoothness on \cora with various attack perturbation rates.} 
    \label{fig:cora-localsmoothness}
\end{figure*}

\begin{figure*}[h!]%
%\vskip -0.2em
     \centering
     \subfloat[0\%]{{\includegraphics[width=0.22\linewidth]{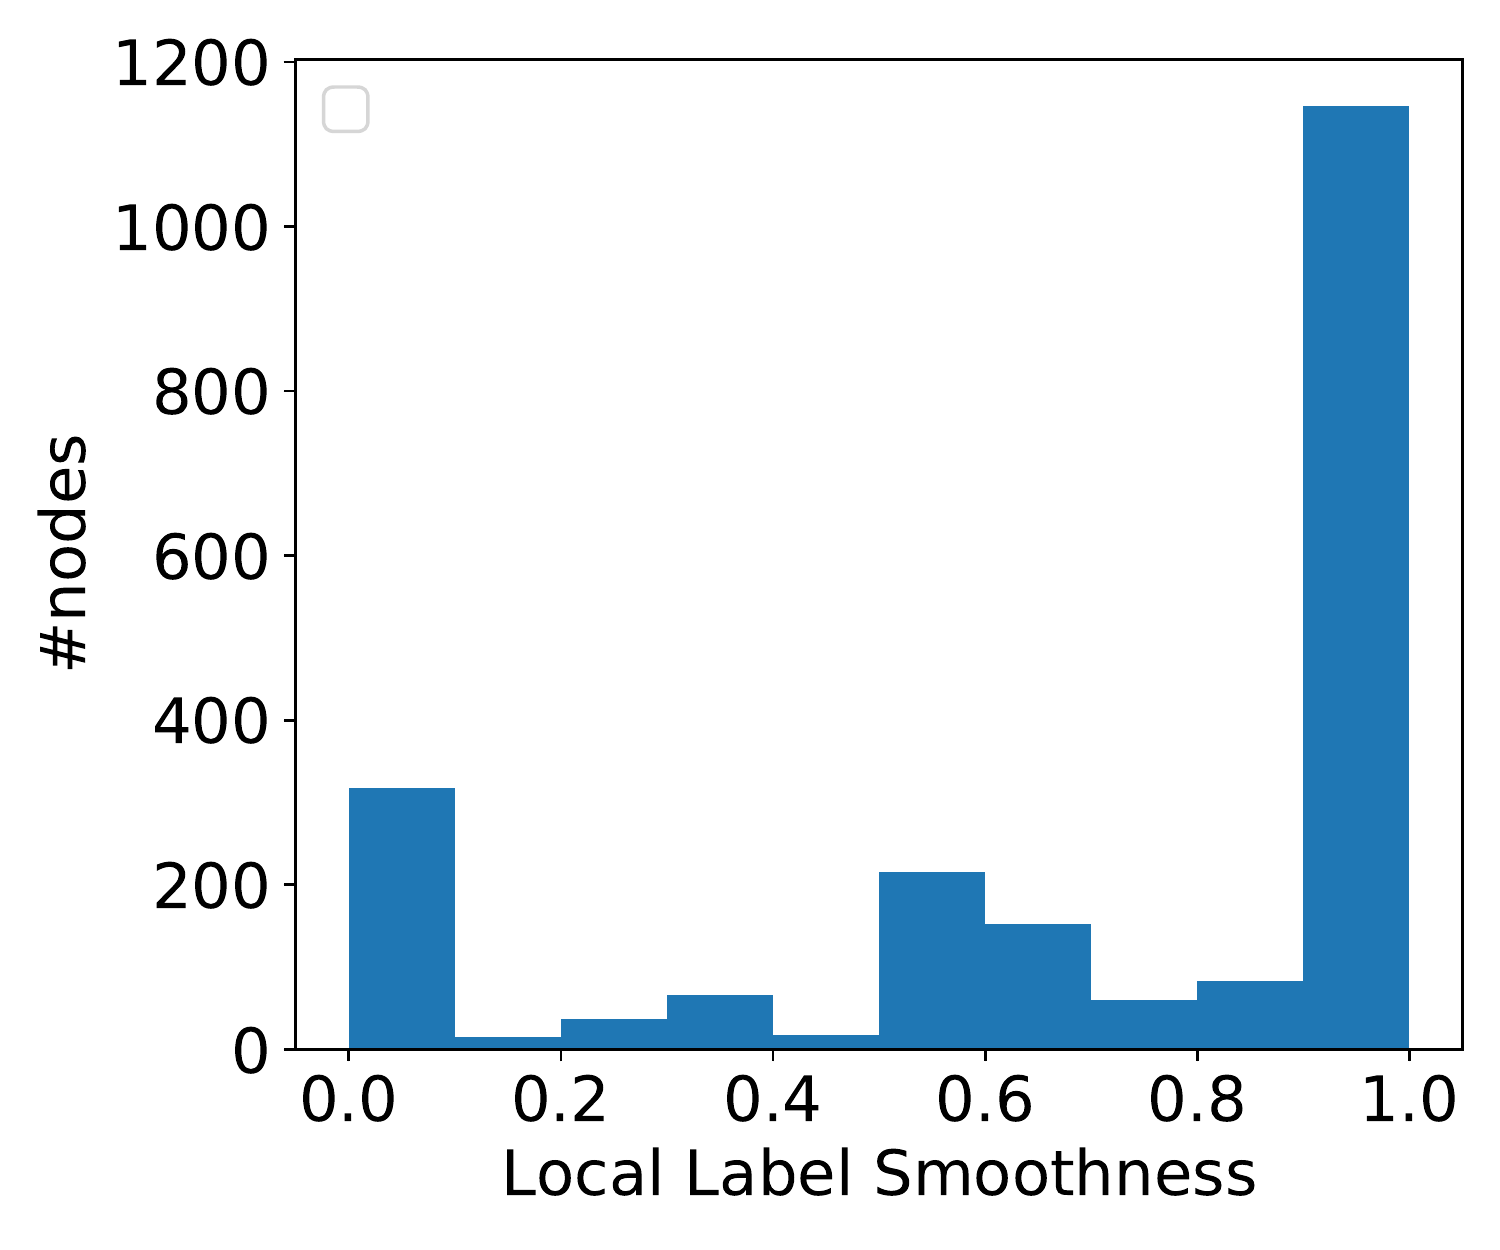} }}%
     \subfloat[5\%]{{\includegraphics[width=0.22\linewidth]{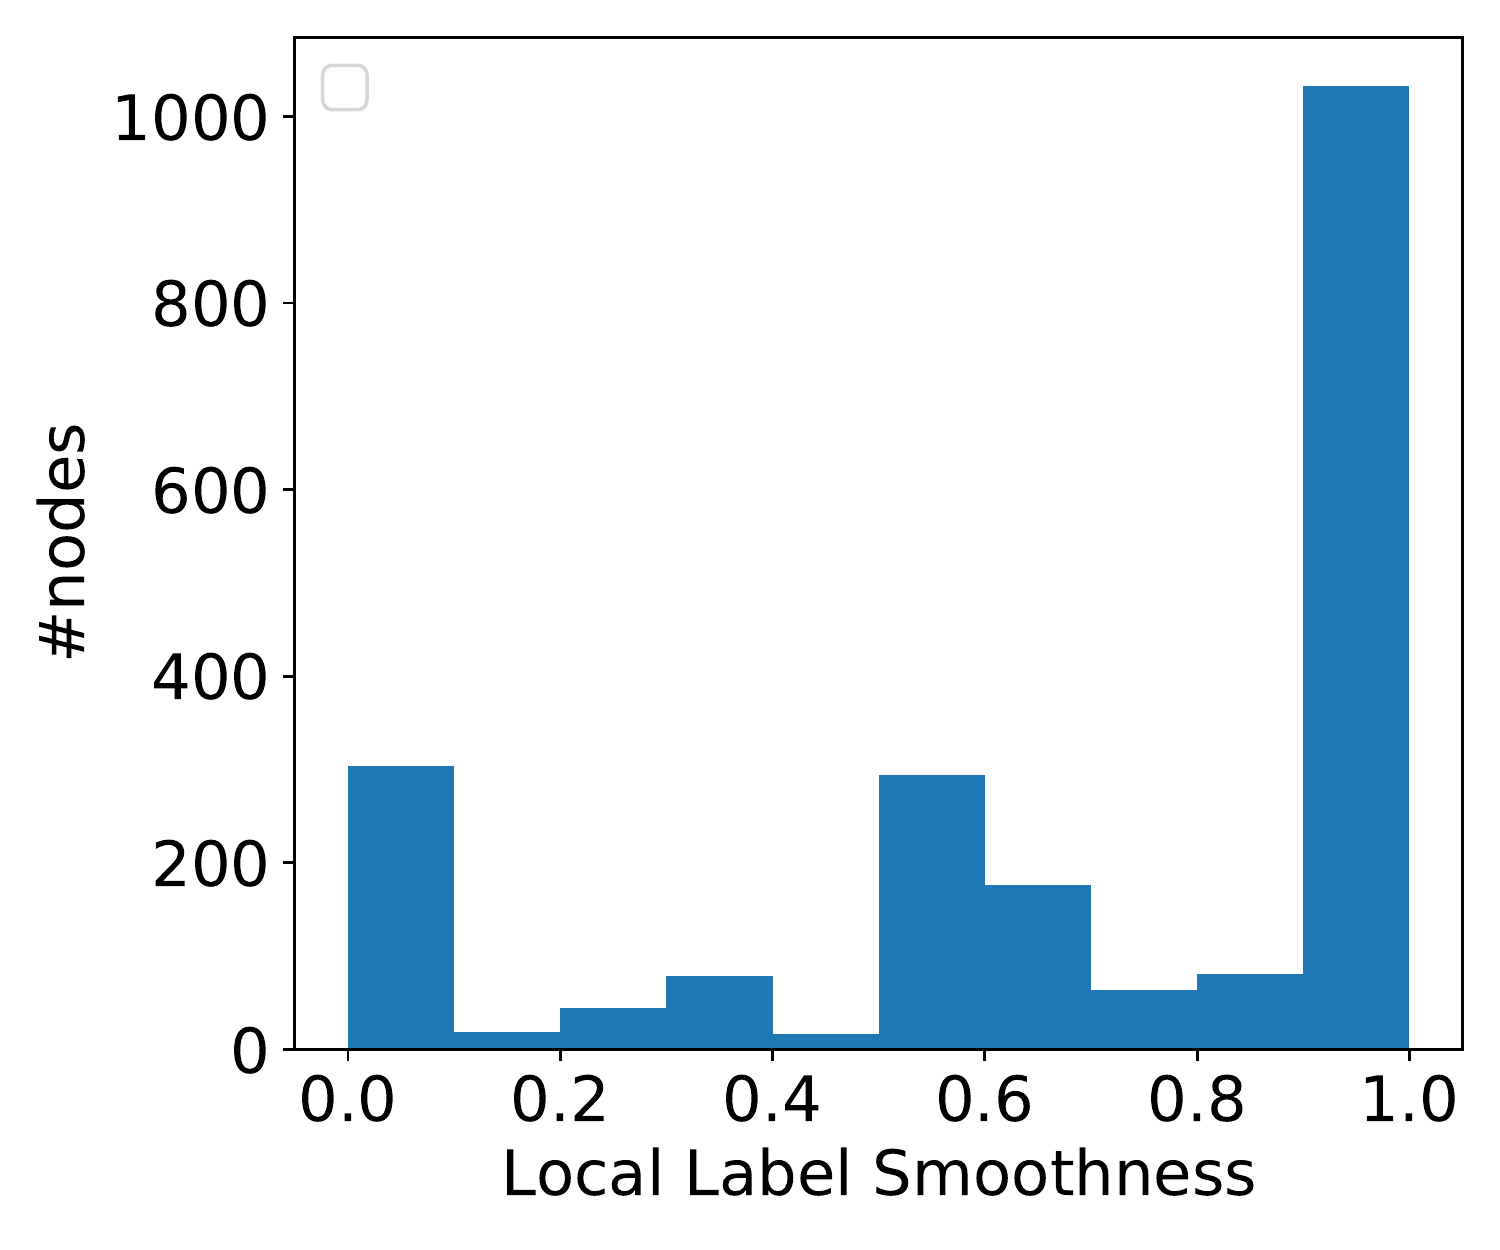} }}%
    \subfloat[15\%]{{\includegraphics[width=0.22\linewidth]{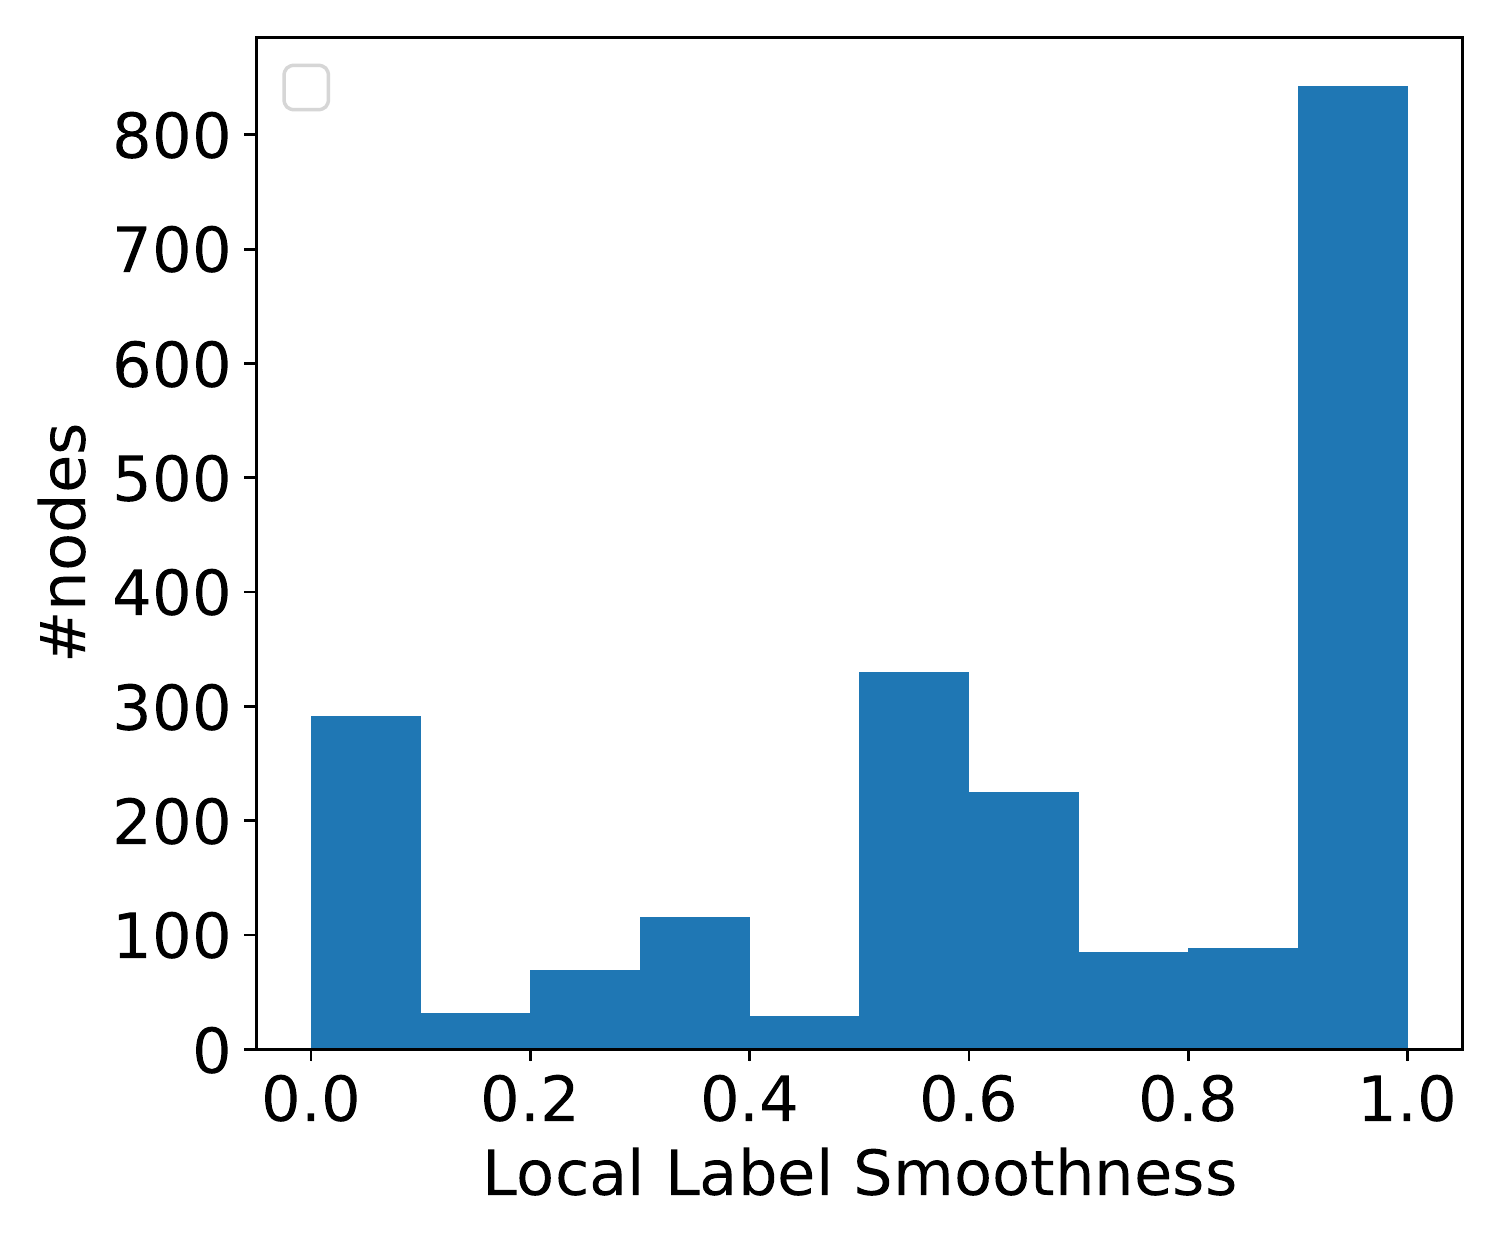} }}%
    \subfloat[25\%]{{\includegraphics[width=0.22\linewidth]{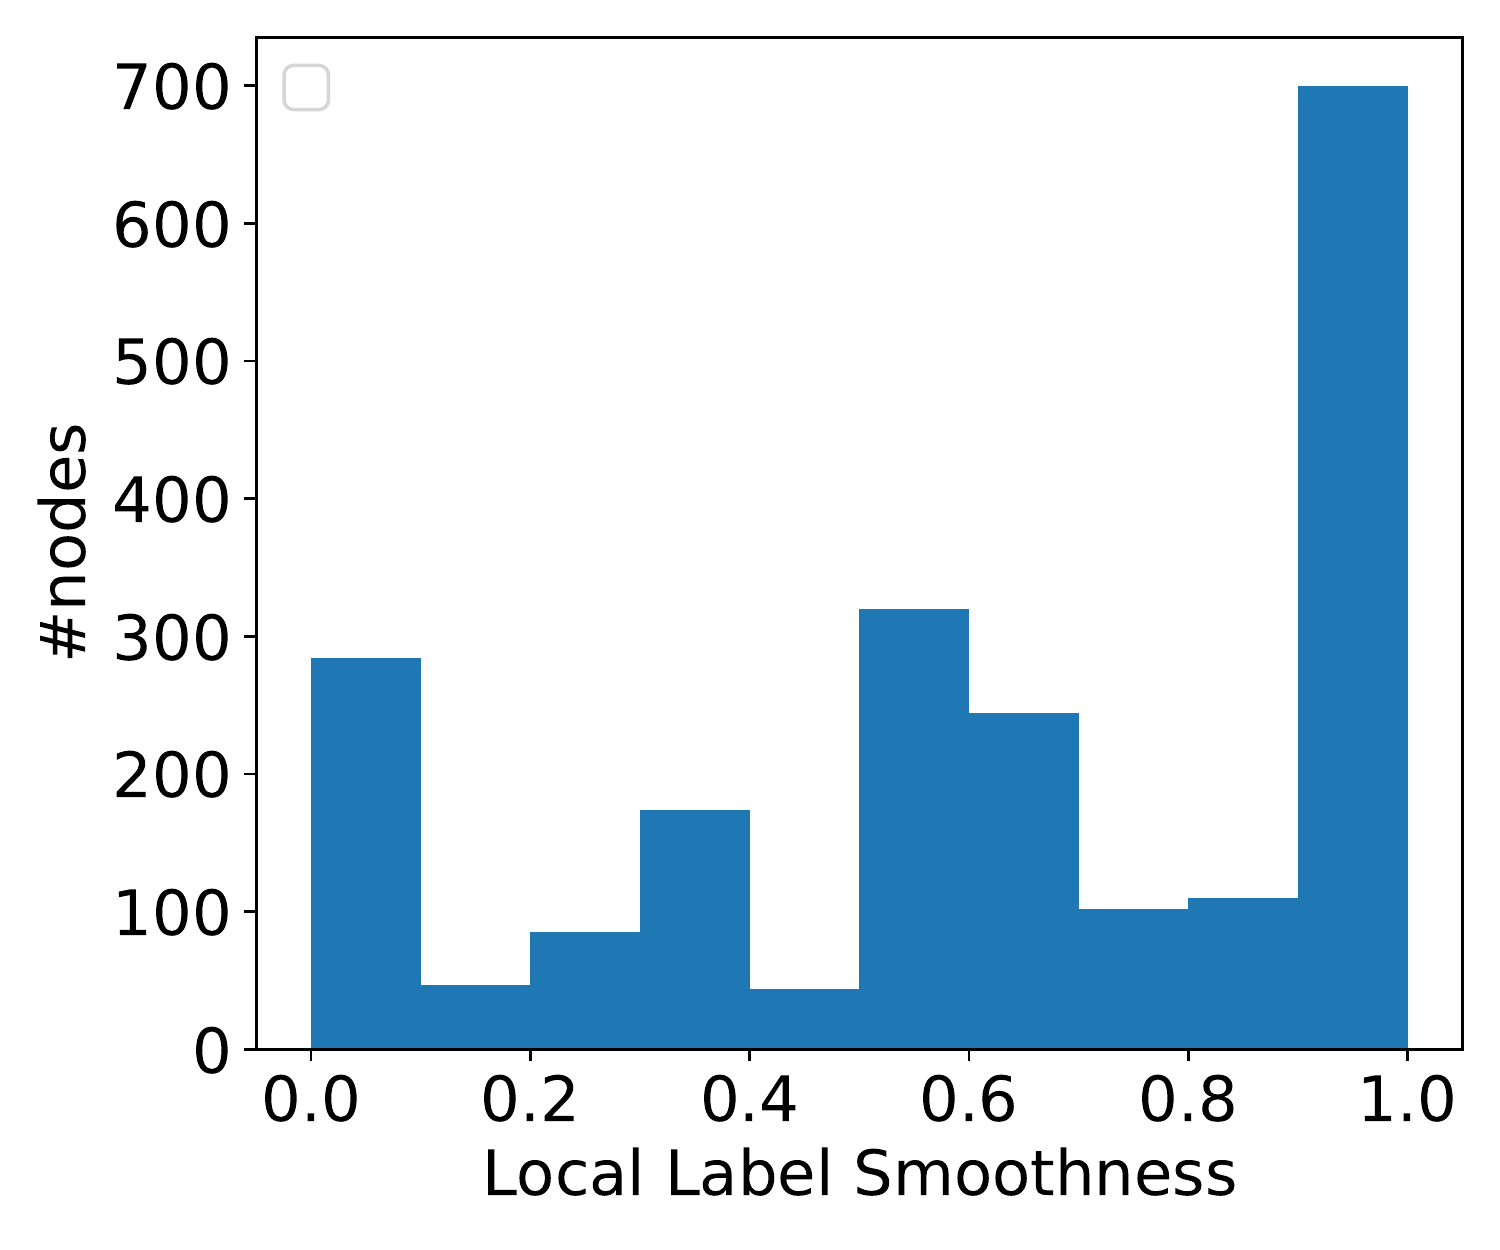} }}%
    \qquad
    \vskip -0.25em
    \caption{Distribution of local label smoothness on \citeseer with various attack perturbation rates.} 
    \label{fig:citeseer-localsmoothness}
\end{figure*}

\begin{figure*}[h!]%
%\vskip -0.2em
     \centering
     \subfloat[0\%]{{\includegraphics[width=0.22\linewidth]{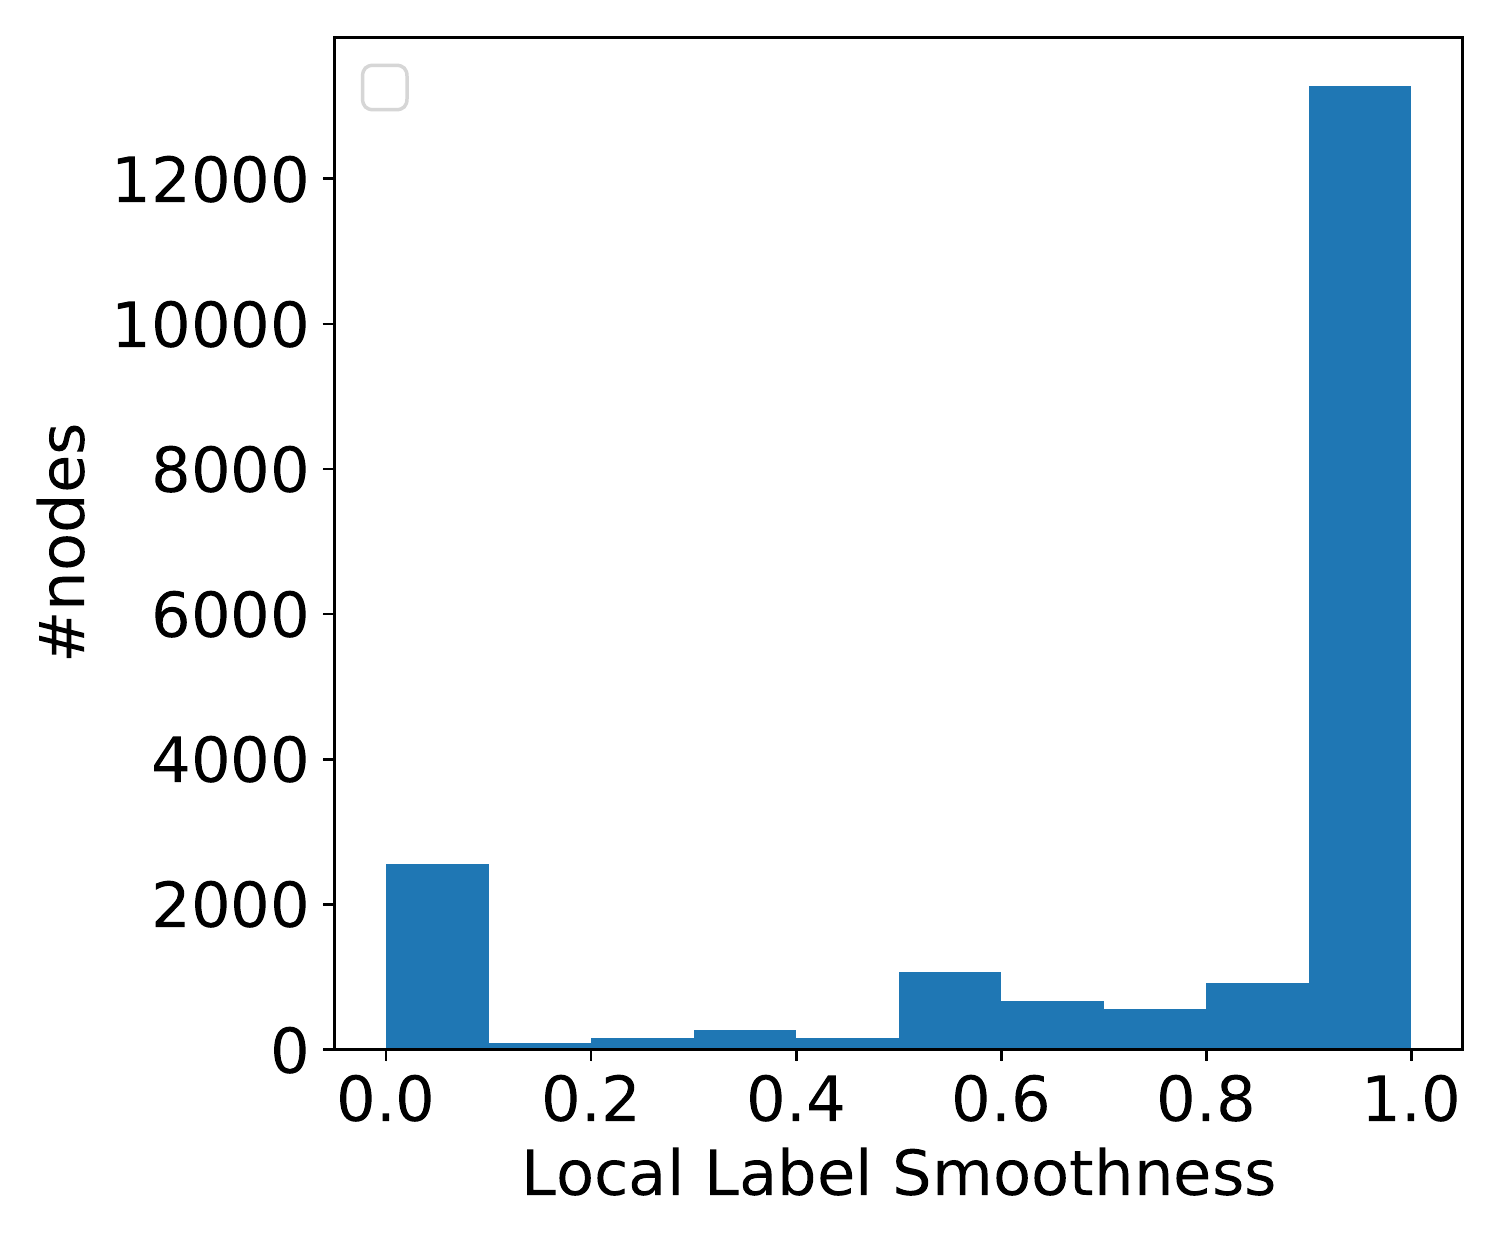} }}%
     \subfloat[5\%]{{\includegraphics[width=0.22\linewidth]{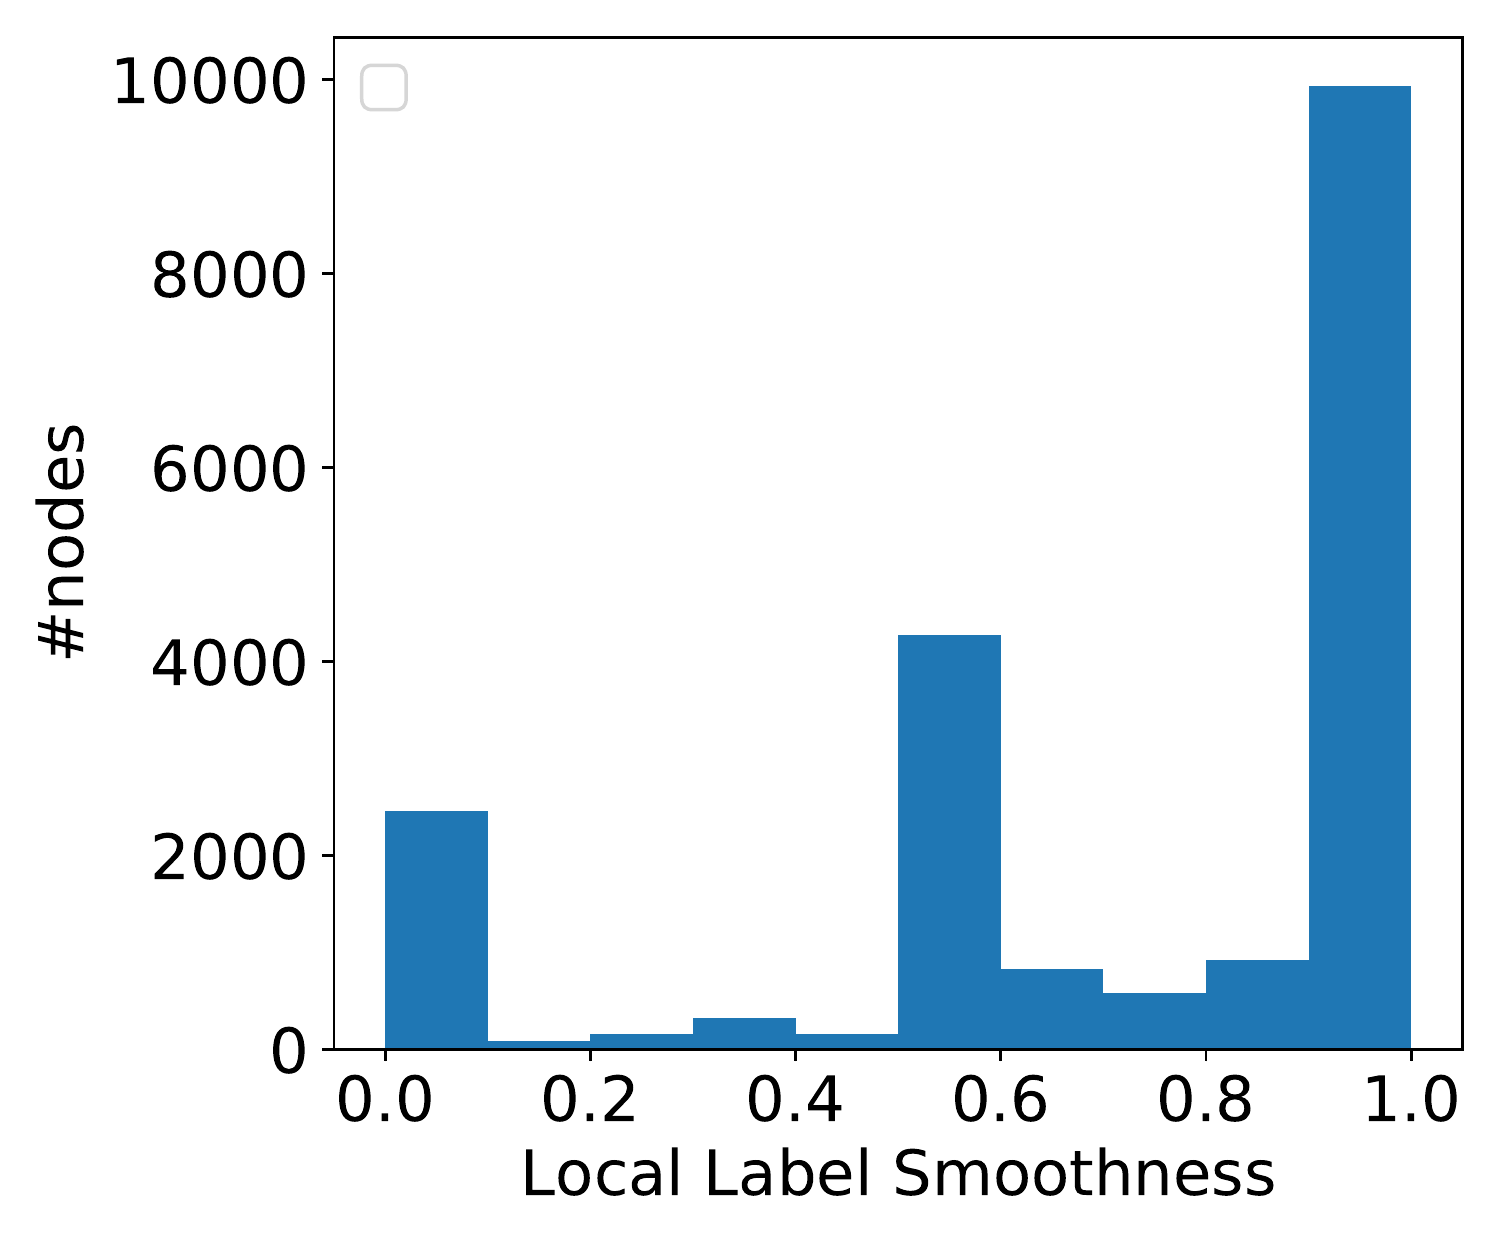} }}%
    \subfloat[15\%]{{\includegraphics[width=0.22\linewidth]{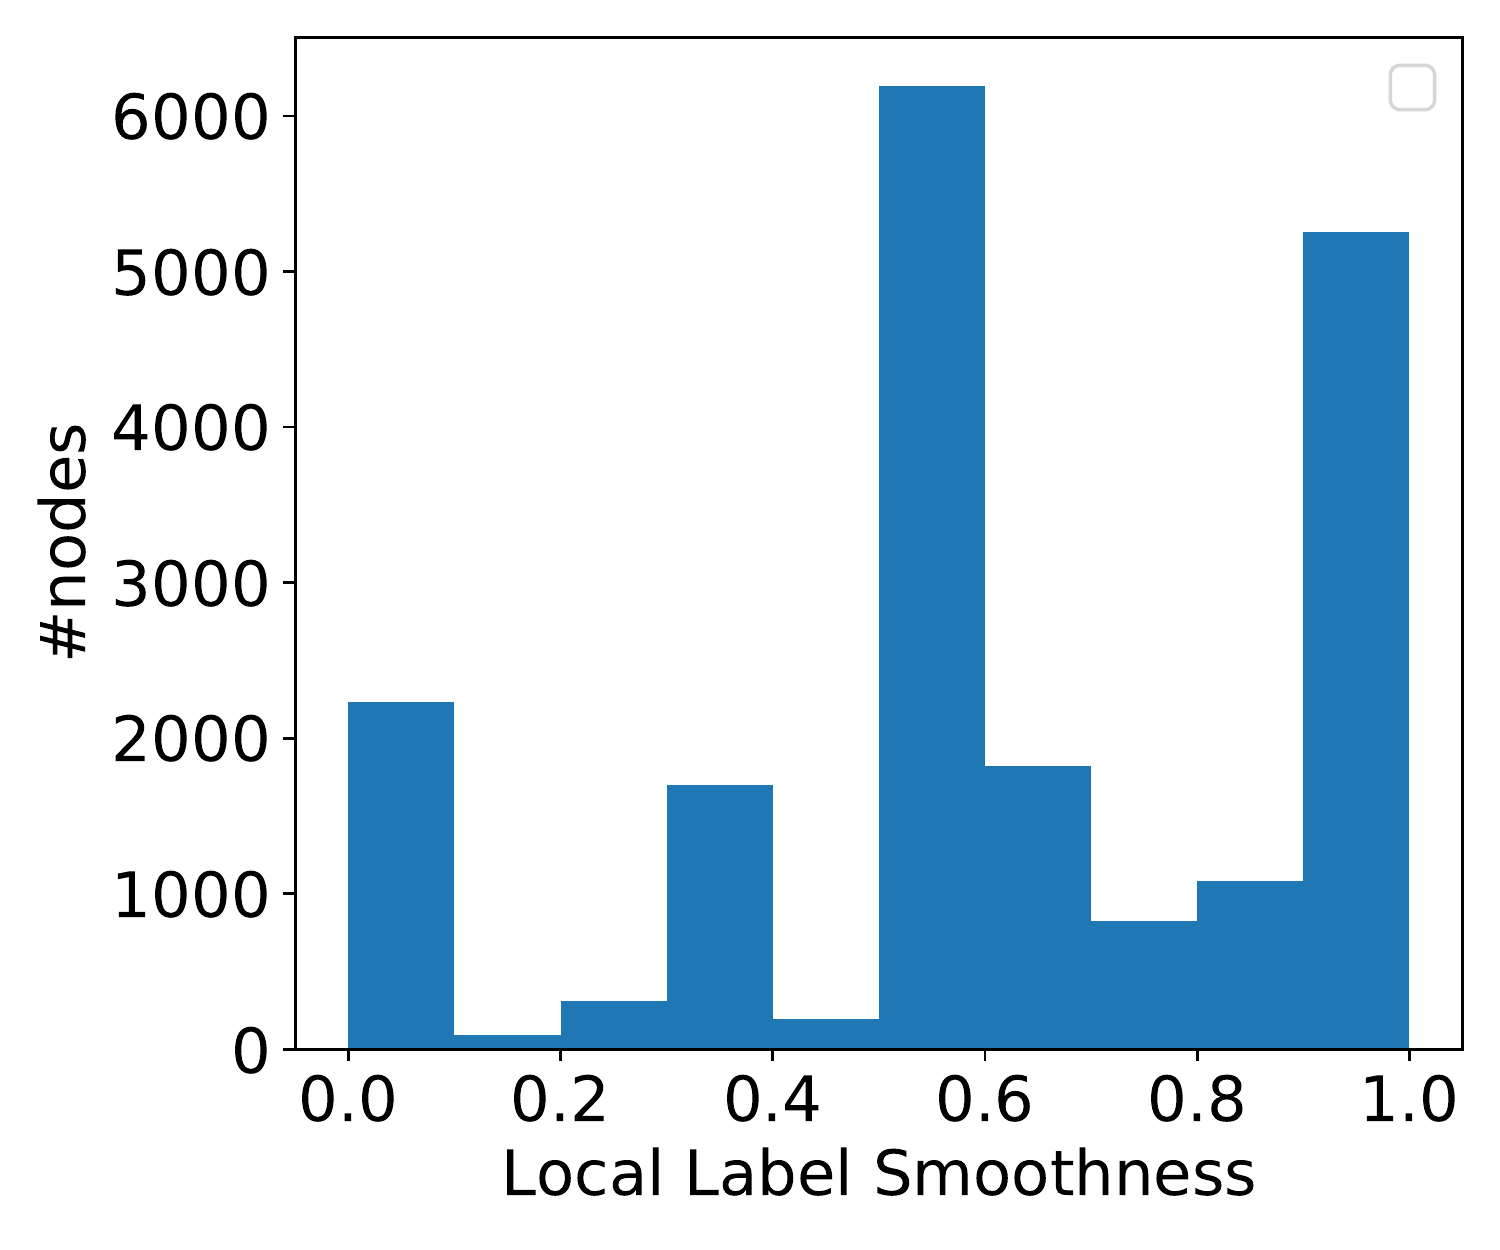} }}%
    \subfloat[25\%]{{\includegraphics[width=0.22\linewidth]{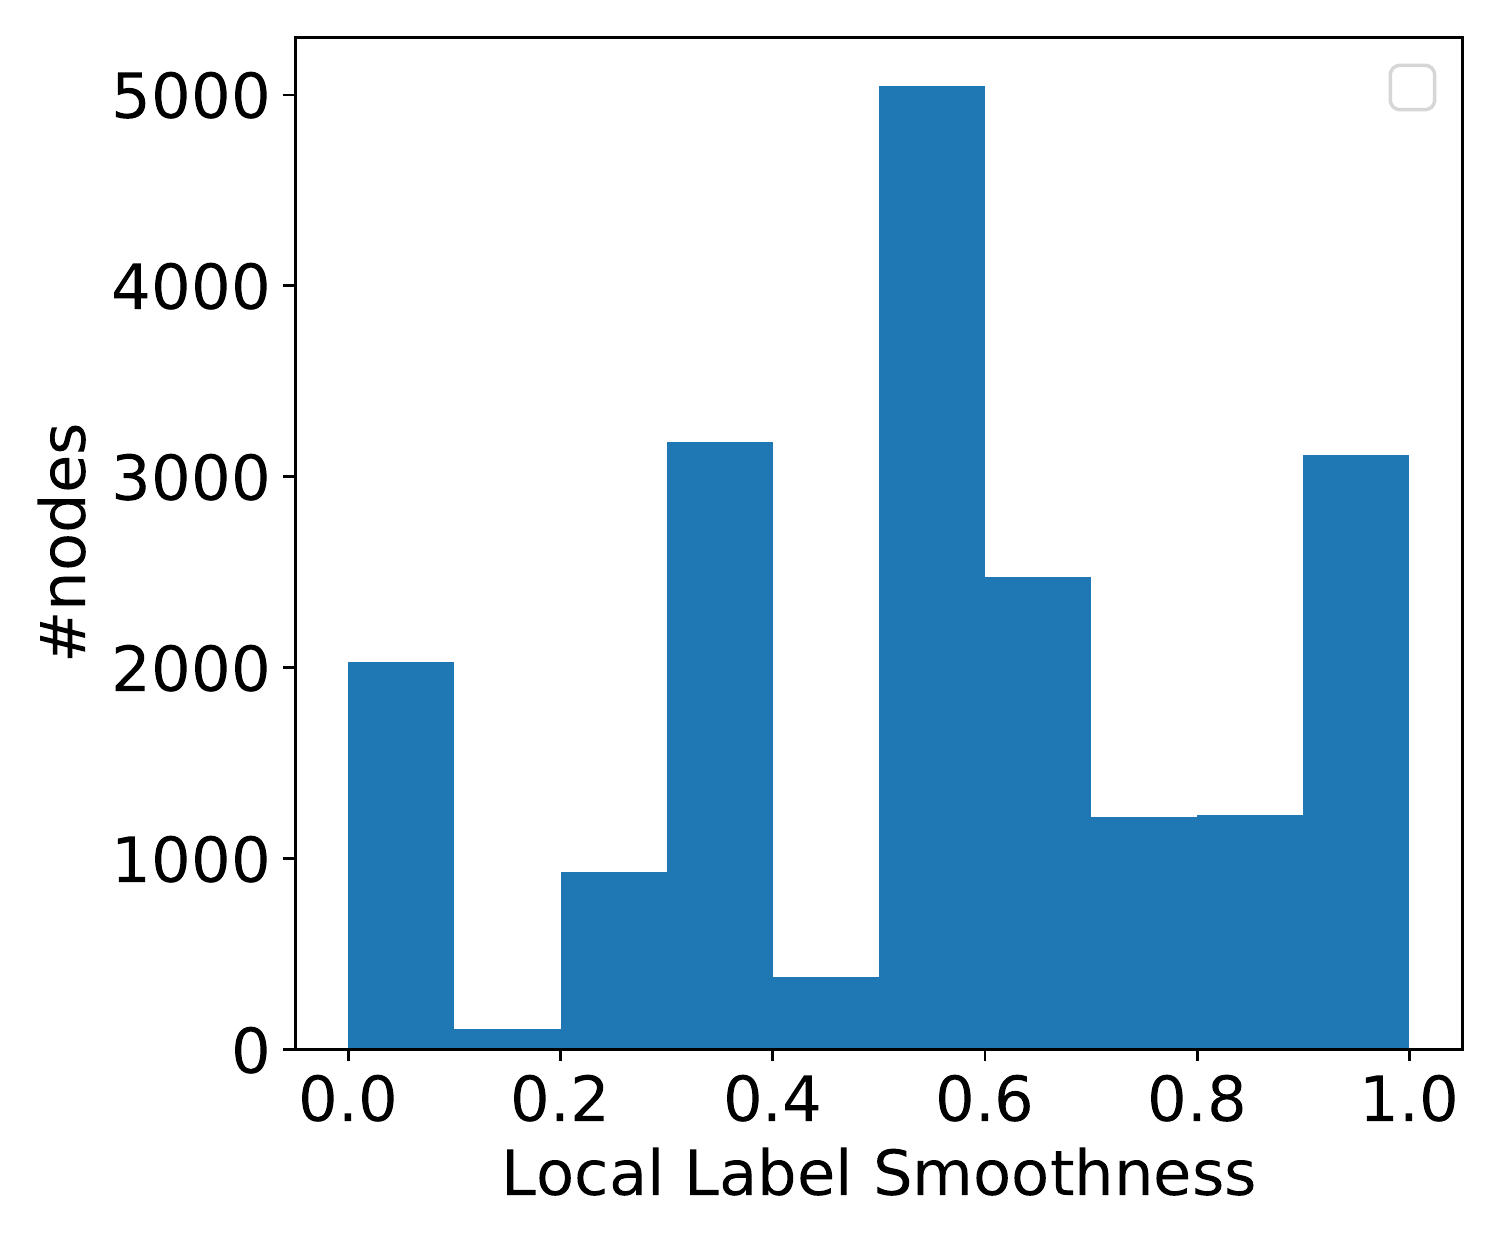} }}%
    \qquad
    \caption{Distribution of local label smoothness on \pubmed with various attack perturbation rates.} 
    \label{fig:pubmed-localsmoothness}
\vskip -0.25em
\end{figure*}

\subsection{More Results on Adversarial Attacks}\label{apx:baseline_for_defense}

We compare our method both with standard GNNs discussed in Section \ref{sec:graph_and_gnn} (GCN, GAT, APPNP), but also with recent state-of-the-art defense techniques against adversarial attacks including GCN-Jaccard~\citep{wu2019adversarial}, GCN-SVD~\citep{entezari2020all}, Pro-GNN-fs and Pro-GNN~\citep{jin2020graph}. The detailed description of these methods are listed as follows:
\begin{compactitem}
        \item {\bf GCN-Jaccard~\citep{wu2019adversarial}:} GCN-Jaccard aims to pre-process a given attacked graph by removing those edges added by the attackers. Specifically, Jaccard smilarlity is utilized to measure the feature similarity between connected pairs of nodes. The edges between node pairs with low-similarity are removed by the algorithm. This pre-processed graph is then utilized for the node classification task.
        \item {\bf GCN-SVD~\citep{entezari2020all}:} GCN-SVD is also a pre-process method. It use SVD to decompose the adjacency matrix of a given perturbed graph and then obtain its low-rank approximation. The low-rank approximation is believed to be cleaner as graph adversarial attacks are observed to be high-rank in ~\citep{entezari2020all}. 
        \item {\bf RGCN~\citep{zhu2019robust}} utilizes Gaussian distributions to model node representations instated of vectors. The Gaussian distributions are expected to absorb the negative impacts from the adversarial attacks and thus achieve more stable performance. 
        \item {\bf Pro-GNN~\citep{jin2020graph}:} Pro-GNN tries to learn a cleaner graph while training the node classification model at the same time. Specifically, it treats the adjacency as parameters, which is optimized during the training stage. Several different constraints are enforced to this learnable adjacency matrix, including: 1) the learned adjacency matrix should be close to the original adjacency matrix; 2) the learned adjacency matrix should be low-rank; and 3) the learned adjacency matrix should ensure feature smoothness. {\bf Pro-GNN-fs} is a variant of Pro-GNN where the third constraint, i.e. feature smoothness, is not enforced. 
\end{compactitem}

Results under varying perturbation rates (attack intensities) are shown in Table~\ref{table:metattack}. Again, we observe that GAT outperforms GCN, suggesting the appeal of an adaptive local smoothness assumption.  Here, our method (orange) substantially outperforms GCN, GAT and APPNP by a large margin, especially in scenarios with high perturbation rate.  %As we can tell from the results, \ym{GAT outperforms GCN, which further demonstrates the necessity to enforce adaptive local smoothness especially for graphs with varying levels of local smoothness.}
%Moreover, compared to APPNP, we , our proposed \methodadaptive is much more robust under adversarial attacks in most of the settings on all three datasets. Especially, when the perturbation rate is large, the proposed \methodadaptive outperforms APPNP with a large margin. 
Moreover, the proposed \methodadaptive is also even more robust than several specially designed adversarial defense methods, like GCN-Jaccard and GCN-SVD, which are based on pre-processing the adversarial attack graphs to obtain cleaner ones, thanks to its adaptive smoothness assumption. Compared with Pro-GNN-fs, our method performs comparably or even better in a few settings, especially when perturbation rate is high. Furthermore, in these settings, the performance of our method is even closer to Pro-GNN, which is the current state-of-the art adversarial defense technique. Note that, Pro-GNN-fs and Pro-GNN involves learning cleaner adjacency matrices of the attacked graphs, and thus has $O(M)$ parameters (M denotes the number of edges in a graph), while our proposed model has far less parameters. Specifically, we have $O(d_{in}\cdot d_{out})$ for feature transformation and $J$ parameters for modeling $h_1(\cdot)$ with $J$ denoting the number of labels. 

\begin{table*}[h!] 
\small
\caption{Robustness under adversarial attacks (node classification accuracy).}
\label{table:metattack}
\begin{threeparttable}
\begin{adjustbox}{width=1\textwidth}
\begin{tabular}{c|c|ccccccccc}
\toprule
Dataset        & Ptb Rate (\%)  & GCN                     & GAT                     & RGCN           & GCN-Jaccard    & GCN-SVD    &APPNP& \methodadaptive     & Pro-GNN-fs              & Pro-GNN                 \\ \midrule
\multirow{6}{*}{Cora}     & 0                                                         & 83.50$\pm$0.44          & 83.97$\pm$0.65 & 83.09$\pm$0.44 & 82.05$\pm$0.51 & 80.63$\pm$0.45 & 85.01$\pm$0.35& 84.38$\pm$ 0.79& 83.42$\pm$0.52          & 82.98$\pm$0.23          \\
                          & 5                                                         & 76.55$\pm$0.79          & 80.44$\pm$0.74          & 77.42$\pm$0.39 & 79.13$\pm$0.59 & 78.39$\pm$0.54 & 79.06$\pm$1.30 & 79.61$\pm$ 0.63 & 82.78$\pm$0.39 & 82.27$\pm$0.45          \\
                          & 10                                                        & 70.39$\pm$1.28          & 75.61$\pm$0.59          & 72.22$\pm$0.38 & 75.16$\pm$0.76 & 71.47$\pm$0.83 &   73.12$\pm$ 0.85& 74.56$\pm$ 0.71&77.91$\pm$0.86         & 79.03$\pm$0.59 \\
                          & 15                                                        & 65.10$\pm$0.71          & 69.78$\pm$1.28          & 66.82$\pm$0.39 & 71.03$\pm$0.64 & 66.69$\pm$1.18 & 71.12$\pm$ 0.97& 72.27$\pm$ 1.10& 76.01$\pm$1.12          & 76.40$\pm$1.27 \\
                          & 20                                                        & 59.56$\pm$2.72          & 59.94$\pm$0.92          & 59.27$\pm$0.37 & 65.71$\pm$0.89 & 58.94$\pm$1.13 & 58.50$\pm$ 1.57& 69.97$\pm$0.74 &68.78$\pm$5.84          & 73.32$\pm$1.56 \\
                          & 25                                                        & 47.53$\pm$1.96          & 54.78$\pm$0.74          & 50.51$\pm$0.78 & 60.82$\pm$1.08 & 52.06$\pm$1.19 & 54.13$\pm$ 1.06& 62.13$\pm$ 0.68&56.54$\pm$2.58          & 69.72$\pm$1.69 \\
\midrule
\multirow{6}{*}{Citeseer} & 0                                                         & 71.96$\pm$0.55          & 73.26$\pm$0.83          & 71.20$\pm$0.83 & 72.10$\pm$0.63 & 70.65$\pm$0.32 &75.92$\pm$ 0.23 & 75.69$\pm$ 0.56& 73.26$\pm$0.38          & 73.28$\pm$0.69 \\
                          & 5                                                         & 70.88$\pm$0.62          & 72.89$\pm$0.83          & 70.50$\pm$0.43 & 70.51$\pm$0.97 & 68.84$\pm$0.72 &  74.13$\pm$ 0.83& 74.28$\pm$ 0.52& 73.09$\pm$0.34 & 72.93$\pm$0.57          \\
                          & 10                                                        & 67.55$\pm$0.89          & 70.63$\pm$0.48          & 67.71$\pm$0.30 & 69.54$\pm$0.56 & 68.87$\pm$0.62 &70.74$\pm$1.18 &71.60$\pm$ 0.36& 72.43$\pm$0.52          & 72.51$\pm$0.75 \\
                          & 15                                                        & 64.52$\pm$1.11          & 69.02$\pm$1.09          & 65.69$\pm$0.37 & 65.95$\pm$0.94 & 63.26$\pm$0.96 & 72.34$\pm$0.99&73.63$\pm$0.99 &70.82$\pm$0.87          & 72.03$\pm$1.11 \\
                          & 20                                                        & 62.03$\pm$3.49          & 61.04$\pm$1.52          & 62.49$\pm$1.22 & 59.30$\pm$1.40 & 58.55$\pm$1.09 & 58.98$\pm$0.83& 66.13$\pm$0.46&66.19$\pm$2.38          & 70.02$\pm$2.28 \\
                          & 25                                                        & 56.94$\pm$2.09          & 61.85$\pm$1.12          & 55.35$\pm$0.66 & 59.89$\pm$1.47 & 57.18$\pm$1.87 & 61.90$\pm$1.48&68.79$\pm$0.43& 66.40$\pm$2.57          & 68.95$\pm$2.78 \\

\midrule
\multirow{6}{*}{Pubmed}   & 0                                                         & 87.19$\pm$0.09          & 83.73$\pm$0.40          & 86.16$\pm$0.18 & 87.06$\pm$0.06 & 83.44$\pm$0.21 &86.59$\pm$ 0.08 &88.17$\pm$0.10& 87.33$\pm$0.18 & 87.26$\pm$0.23          \\
                          & 5                                                         & 83.09$\pm$0.13          & 82.87$\pm$0.18          & 81.08$\pm$0.20 & 86.39$\pm$0.06 & 83.41$\pm$0.15 & 84.67$\pm$0.10&87.62$\pm$0.17&87.25$\pm$0.09 & 87.23$\pm$0.13          \\
                          & 10                                                        & 81.21$\pm$0.09          & 81.29$\pm$0.33          & 77.51$\pm$0.27 & 85.70$\pm$0.07 & 83.27$\pm$0.21 &83.59$\pm$0.11 &87.17$\pm$0.12& 87.25$\pm$0.09 & 87.21$\pm$0.13          \\
                          & 15                                                        & 78.66$\pm$0.12          & 79.62$\pm$0.43          & 73.91$\pm$0.25 & 84.76$\pm$0.08 & 83.10$\pm$0.18 &81.98$\pm$ 0.24 &86.68$\pm$0.11& 87.20$\pm$0.09 & 87.20$\pm$0.15          \\
                          & 20                                                        & 77.35$\pm$0.19          & 77.43$\pm$0.32          & 71.18$\pm$0.31 & 83.88$\pm$0.05 & 83.01$\pm$0.22 & 81.35$\pm$0.15 &86.49$\pm$0.11& 87.09$\pm$0.10          & 87.15$\pm$0.15 \\
                          & 25                                                        & 75.50$\pm$0.17          & 75.46$\pm$0.68          & 67.95$\pm$0.15 & 83.66$\pm$0.06 & 82.72$\pm$0.18 & 80.84$\pm$0.08&86.01$\pm$0.07& 86.71$\pm$0.09          & 86.76$\pm$0.19 \\ %\cmidrule(l){2-9} 
\bottomrule
\end{tabular}
\end{adjustbox}
\end{threeparttable}

\end{table*}
