# Supplementary material for: A Unified View on Graph Neural Networks as Graph Signal Denoising
Source: arXiv:2010.01777 source file (2021-10-18)
Supplement: Supplementary file 3 [file appendix_pairnorm.tex]

\section{Connections to PairNorm and DropEdge}\label{apx:parinorm}
PairNorm and DropEdge, which are two recently proposed GNN enhancements for developing deeper GNN models, are corresponding to the following regularization terms:
\begin{align}
    &\text{PairNorm: }   \sum\limits_{(i,j) \in \mathcal{E}} \mathcal{C}_p \cdot \left\| {\bf F}_i - {\bf F}_j\right\|_2^2 -  \sum\limits_{(i,j) \not\in \mathcal{E}} \mathcal{C}_n \cdot \left\| {\bf F}_i - {\bf F}_j\right\|_2^2, \label{eq:reg_pair_norm}\\
    & \text{DropEdge: }  \sum\limits_{(i,j) \in \mathcal{E}} \mathcal{C}_{ij} \cdot \left\| {\bf F}_i - {\bf F}_j\right\|_2^2, \ \text{where} \ \mathcal{C}_{ij}\in \{0,1\}. \label{eq:reg_dropedge}
\end{align}
% \ns{need to mention we show these in appendix; not obvious}
For PairNorm, $\mathcal{C}$ consists of $\mathcal{C}_p, \mathcal{C}_n>0$ and the regularization term ensures connected nodes to be similar while disconnected nodes to be dissimilar. For DropEdge, $\mathcal{C}$ is a sparse matrix having the same shape as adjacency matrix. For each edge $(i,j)$, its corresponding $\mathcal{C}_{ij}$ is sampled from a Bernoulli distribution with mean $1-q$, where $q$ is a pre-defined dropout rate.
