# Supplementary material for: A Unified View on Graph Neural Networks as Graph Signal Denoising
Source: arXiv:2010.01777 source file (2021-10-18)
Supplement: Supplementary file 4 [file appendix_proof.tex]

\section{Proofs}
